# Supplementary material for: Quantum Linear Time-Translation-Invariant Systems: Conjugate Symplectic Structure, Uncertainty Bounds, and Tomography
Source: arXiv:2410.09976 ancillary file (2024-10-15)
Supplement: Supplementary file 1 [file SI.pdf]

# Supplementary Information for “Quantum Linear Time-Translation-Invariant Systems: Conjugate Symplectic Structure, Uncertainty Bounds, and Tomography”

Jacques Ding,<sup>1,2</sup> Hudson A. Loughlin,<sup>1</sup> and Vivishek Sudhir<sup>1,3</sup>

<sup>1</sup>*LIGO Laboratory, Massachusetts Institute of Technology, Cambridge, MA 02139*

<sup>2</sup>*Laboratoire Astroparticule et Cosmologie, Université Paris Cité, Paris, 75000, France*

<sup>3</sup>*Department of Mechanical Engineering, Massachusetts Institute of Technology, Cambridge, MA 02139*

(Dated: October 13, 2024)

## CONTENTS

|                                                                                                                           |    |
|---------------------------------------------------------------------------------------------------------------------------|----|
| I. Inertia of hermitian matrices and proof of the minimum number of noise modes (Theorem 1 of main text)                  | 3  |
| A. Inertia theorems                                                                                                       | 3  |
| B. Proof of Theorem 1 of main text                                                                                        | 4  |
| II. Proof of the conjugate-symplectic dilation theorem (Section II C of main text)                                        | 4  |
| III. Proof of the optical decomposition (Theorem 2 of main text)                                                          | 5  |
| A. The conjugate symplectic SVD                                                                                           | 6  |
| 1. Properties of hermitian conjugate symplectic matrices                                                                  | 6  |
| 2. The spectral theorem for $\text{HPD} \cap \text{Sp}^\dagger(2n)$                                                       | 7  |
| 3. Proof of conjugate symplectic SVD                                                                                      | 9  |
| B. The conjugate symplectic CSD                                                                                           | 10 |
| C. Relationship with KAK decomposition                                                                                    | 11 |
| IV. Relation between $\text{Sp}^\dagger(2n)$ and $\text{Sp}(4n, \mathbb{R})$ (Section III C of main text)                 | 11 |
| A. A pair of harmonic oscillators for each frequency                                                                      | 12 |
| 1. Introduction for a single mode $\hat{a}[\omega]$                                                                       | 12 |
| 2. General, multimode case: doubled forms                                                                                 | 13 |
| B. Input and output relations                                                                                             | 13 |
| 1. Real form of a complex matrix                                                                                          | 13 |
| 2. Formal approach                                                                                                        | 14 |
| C. Physical interpretation of $\text{Sp}^\dagger(2n) \neq \mathfrak{Sp}(4n, \mathbb{R})$                                  | 15 |
| D. Physical detectability of the bona fide quadratures $\hat{\mathfrak{X}}[\omega]$                                       | 15 |
| 1. Synodyne measurement of the bona fide quadratures                                                                      | 15 |
| 2. Spectral correlations of the bona fide quadratures                                                                     | 16 |
| V. Proof of the uncertainty principle (Theorem 3 of main text) and consequences                                           | 16 |
| VI. Proof of the conjugate symplectic reduction of the SDM (Theorem 4 of main text)                                       | 17 |
| A. Conjugate symplectic reduction for a hermitian positive definite matrix                                                | 17 |
| B. Proof of Theorem 4 of main text                                                                                        | 19 |
| VII. Proof of the tighter uncertainty bound for open LTI systems (Theorem 5 of main text)                                 | 20 |
| VIII. The synodyne detection local oscillator as an example of quadrature amplitude modulation (Section V A of main text) | 21 |
| A. Quadrature amplitude modulation                                                                                        | 21 |
| B. Connection with the synodyne local oscillator                                                                          | 22 |
| IX. An example of a frequency-dependent two-mode beamsplitter (Section VI A of main text)                                 | 22 |
| X. Details of complex squeezing in lossy passive systems (Section VI B of main text)                                      | 23 |
| A. Derivation of the output SDM of equation 64 in main text                                                               | 23 |
| B. Full expressions of the eigenvalues $\Lambda_-^{\mathbb{R}, \mathbb{C}}$                                               | 23 |
| C. Validity of the approximation of main text Eq. 66                                                                      | 24 |

|                                                        |    |
|--------------------------------------------------------|----|
| D. Choosing the parameters for a detuned filter cavity | 25 |
| XI. Details of appendix A of main text                 | 25 |
| References                                             | 26 |

# I. INERTIA OF HERMITIAN MATRICES AND PROOF OF THE MINIMUM NUMBER OF NOISE MODES (THEOREM 1 OF MAIN TEXT)

## A. Inertia theorems

In this section we summarize results related to Sylvester's law of inertia [1, 2]. We first define the notions of matrix congruence and inertia.

**Definition 1.** Two hermitian matrices  $\mathbf{A}, \mathbf{B} \in \mathcal{M}_n(\mathbb{C})$  are congruent if there exists an invertible matrix  $\mathbf{S} \in \mathcal{M}_n(\mathbb{C})$  such that

$$\mathbf{A} = \mathbf{S}\mathbf{B}\mathbf{S}^\dagger \quad (\text{I.1})$$

It is straightforward to check that the matrix congruence is an equivalence relation.

**Definition 2.** The inertia of a Hermitian matrix  $\mathbf{A} \in \mathcal{M}_n(\mathbb{C})$  is the triplet  $(n_+, n_-, n_0)$  of non-negative integers, where  $n_+$  (resp.  $n_-$ ,  $n_0$ ) is the number of positive (resp. negative, zero) eigenvalues of  $\mathbf{A}$ , counting multiplicity. We denote the inertia of a matrix by  $\text{In}(\mathbf{A}) = (n_+(\mathbf{A}), n_-(\mathbf{A}), n_0(\mathbf{A}))$ .

Sylvester's law of inertia can then be stated as follows:

**Theorem 1.** Let  $\mathbf{A}, \mathbf{B} \in \mathcal{M}_n(\mathbb{C})$  two hermitian matrices. Then,  $\mathbf{A}$  and  $\mathbf{B}$  are congruent if and only if they have the same inertia.

**Proposition 1.** Let  $\mathbf{A}, \mathbf{B} \in \mathcal{M}_n(\mathbb{C})$  two hermitian matrices. If  $\mathbf{A}$  and  $\mathbf{B}$  are congruent, and  $\mathbf{A}$  is hermitian positive (semi) definite, then  $\mathbf{B}$  is also hermitian positive (semi) definite.

The following theorem allows us to relate the inertia of a partitioned matrix to the inertias of its submatrices.

**Theorem 2.** If  $\mathbf{H}$  is a Hermitian matrix partitioned as

$$\mathbf{H} = \begin{bmatrix} \mathbf{H}^{11} & \mathbf{H}^{12} \\ \mathbf{H}^{21} & \mathbf{H}^{22} \end{bmatrix}, \quad (\text{I.2})$$

where  $\mathbf{H}^{11}$  is non-singular, then (see Theorem 1 of ref. [3])

$$\text{In}(\mathbf{H}) = \text{In}(\mathbf{H}^{11}) + \text{In}\left(-\mathbf{H}^{12\dagger} (\mathbf{H}^{11})^{-1} \mathbf{H}^{12}\right) \quad (\text{I.3})$$

A useful corollary of this theorem occurs when  $\mathbf{H}^{12} = \mathbf{H}^{22} = \mathbf{0}$ .

**Theorem 3.** If  $\mathbf{H}$  is a Hermitian matrix partitioned as

$$\mathbf{H} = \begin{bmatrix} \mathbf{H}^{11} & \mathbf{0} \\ \mathbf{0} & \mathbf{0} \end{bmatrix}, \quad (\text{I.4})$$

where  $\mathbf{H}^{11}$  is non-singular, then

$$\text{In}(\mathbf{H}) = \text{In}(\mathbf{H}^{11}) + \text{In}(\mathbf{0}), \quad (\text{I.5})$$

and

$$n_{\pm}(\mathbf{H}) = n_{\pm}(\mathbf{H}^{11}). \quad (\text{I.6})$$

An additional useful theorem relating the eigenvalues of a matrix to its partitions is as follows.

**Theorem 4.** Suppose  $\mathbf{K}$  is a principal submatrix of order  $k$  of the Hermitian matrix  $\mathbf{H}$  of order  $n$ . Then (see Theorem 6 of ref. [3])

$$n_{\pm}(\mathbf{H}) \geq n_{\pm}(\mathbf{K}). \quad (\text{I.7})$$

### B. Proof of Theorem 1 of main text

Using Theorems 1, 3 and 4, we can prove Theorem 1 in the main text as follows. First, we perform a singular value decomposition on  $\mathbf{N}[\omega]$  such that

$$\mathbf{N}[\omega] = \mathbf{V}[\omega] \mathbf{\Sigma}[\omega] \mathbf{W}[\omega], \quad (\text{I.8})$$

where  $\mathbf{V}$  and  $\mathbf{W}$  are unitary matrices, and  $\mathbf{\Sigma}$  is a rectangular matrix with nonzero real entries on the diagonal (the singular values of  $\mathbf{N}$ ) and all other entries equal to zero.

Applying Theorem 1 to  $\mathbf{N}[\omega] \mathbf{iJ}^N \mathbf{N}[\omega]^\dagger$ , we see that

$$n_\pm \left( \mathbf{N}[\omega] \mathbf{iJ}^N \mathbf{N}[\omega]^\dagger \right) = n_\pm \left( \mathbf{\Sigma}[\omega] \mathbf{W}[\omega] \mathbf{iJ}^N \mathbf{W}[\omega]^\dagger \mathbf{\Sigma}[\omega]^\dagger \right). \quad (\text{I.9})$$

Applying Theorems 3 and 4, we have

$$n_\pm \left( \mathbf{\Sigma}[\omega] \mathbf{W}[\omega] \mathbf{iJ}^N \mathbf{W}[\omega]^\dagger \mathbf{\Sigma}[\omega]^\dagger \right) \leq n_\pm \left( \mathbf{W}[\omega] \mathbf{iJ}^N \mathbf{W}[\omega]^\dagger \right), \quad (\text{I.10})$$

and applying Theorem 1 again, we have

$$n_\pm \left( \mathbf{W}[\omega] \mathbf{iJ}^N \mathbf{W}[\omega]^\dagger \right) = k, \quad (\text{I.11})$$

where  $k$  is the number of noise modes and  $\mathbf{J}^N$  is a  $2k \times 2k$  matrix. Combining these results, we have

$$n_\pm \left( \mathbf{N}[\omega] \mathbf{iJ}^N \mathbf{N}[\omega]^\dagger \right) \leq k, \quad (\text{I.12})$$

so the matrix  $\mathbf{N}[\omega] \mathbf{iJ}^N \mathbf{N}[\omega]^\dagger$  cannot have  $\ell$  positive or negative eigenvalues if  $k < \ell$ , which proves Theorem 1 in the main text.

## II. PROOF OF THE CONJUGATE-SYMPLECTIC DILATION THEOREM (SECTION II C OF MAIN TEXT)

Here, we prove a complex version of the symplectic dilation theorem as given in Lemma 1 of ref. [4] and used in Section II C of main text.

**Theorem 5.** *For the  $2n \times 2n$  symplectic form  $\mathbf{J}_{2n}$ , a  $2m \times 2n$  complex matrix  $\mathbf{M}_1$ , and a  $2m \times 2k$  complex matrix  $\mathbf{M}_2$  such that*

$$\mathbf{M}_1 \mathbf{J}_{2n} \mathbf{M}_1^\dagger + \mathbf{M}_2 \mathbf{J}_{2k} \mathbf{M}_2^\dagger = \mathbf{J}_{2m} \quad (\text{II.1})$$

*where  $n + k \geq m$ , we can always find a  $2(n + k - m) \times 2n$  matrix  $\mathbf{M}_3$  and a  $2(n + k - m) \times 2k$  matrix  $\mathbf{M}_4$  such that the  $2(n + k) \times 2(n + k)$  matrix  $\mathbf{M}$ , defined by*

$$\mathbf{M} := \begin{bmatrix} \mathbf{M}_1 & \mathbf{M}_2 \\ \mathbf{M}_3 & \mathbf{M}_4 \end{bmatrix} \quad (\text{II.2})$$

*satisfying*

$$\mathbf{M} \mathbf{J}^{ext} \mathbf{M}^\dagger = \mathbf{J}^{ext}, \quad \text{where} \quad \mathbf{J}^{ext} := \begin{bmatrix} \mathbf{J}_{2m} & \mathbf{0} \\ \mathbf{0} & \mathbf{J}_{2(n+k-m)} \end{bmatrix}. \quad (\text{II.3})$$

*Proof.* This theorem is mathematically equivalent to the following problem: Given  $m$  pairs of column vectors in  $\mathbb{C}^{2(n+k)}$   $\mathbf{q}_1, \dots, \mathbf{q}_m$  and  $\mathbf{p}_1, \dots, \mathbf{p}_m$  that satisfy

$$\begin{aligned} \mathbf{q}_i^\dagger \mathbf{J}_{2(n+k)} \mathbf{q}_j &= 0 \\ \mathbf{p}_i^\dagger \mathbf{J}_{2(n+k)} \mathbf{p}_j &= 0 \\ \mathbf{q}_i^\dagger \mathbf{J}_{2(n+k)} \mathbf{p}_j &= \delta_{ij} \end{aligned} \quad (\text{II.4})$$

for  $i, j = 1, \dots, m$ , find vectors  $\mathbf{q}_{m+1}, \dots, \mathbf{q}_{n+k}$  and  $\mathbf{p}_{m+1}, \dots, \mathbf{p}_{n+k}$  such that

$$\begin{aligned} \mathbf{q}_i^\dagger \mathbf{J}_{2(n+k)} \mathbf{q}_j &= 0 \\ \mathbf{p}_i^\dagger \mathbf{J}_{2(n+k)} \mathbf{p}_j &= 0 \\ \mathbf{q}_i^\dagger \mathbf{J}_{2(n+k)} \mathbf{p}_j &= \delta_{ij} \end{aligned} \quad (\text{II.5})$$

for all  $i, j > m$  and

$$\begin{aligned} \mathbf{q}_i^\dagger \mathbf{J}_{2(n+k)} \mathbf{q}_j &= 0 \\ \mathbf{p}_i^\dagger \mathbf{J}_{2(n+k)} \mathbf{p}_j &= 0 \end{aligned} \quad (\text{II.6})$$

for all  $i > m$  and  $1 \leq j \leq m$ .

To do this, we define the vector space  $V_m := \text{span}(\mathbf{q}_1, \dots, \mathbf{q}_m, \mathbf{p}_1, \dots, \mathbf{p}_m)$  and its complement

$$V_m^\perp := \{\mathbf{x} : \mathbf{x}^\dagger \mathbf{J}_{2(n+k)} \mathbf{y} = 0 \quad \forall \mathbf{y} \in V_m\}. \quad (\text{II.7})$$

We can see that  $V_m \cap V_m^\perp = \{0\}$  because if  $\mathbf{x} \in V_m$  and  $\mathbf{x} \neq 0$ , then  $\mathbf{x}^\dagger \mathbf{J}_{2(n+k)} \mathbf{y} \neq 0$  for some  $\mathbf{y} \in V_m$ , but if  $\mathbf{x} \in V_m^\perp$ , then  $\mathbf{x}^\dagger \mathbf{J}_{2(n+k)} \mathbf{y} = 0 \quad \forall \mathbf{y} \in V_m$ , thus  $\mathbf{x}$  cannot be an element of both  $V_m$  and  $V_m^\perp$  unless  $\mathbf{x} = 0$ .

It is also the case that  $\mathbb{C}^{2(n+k)} = V_m \oplus V_m^\perp$ . We can see this by decomposing a vector  $\mathbf{x} \in \mathbb{C}^{2(n+k)}$  as

$$\mathbf{x} = \left[ \sum_{i=1}^m (-\alpha_i \mathbf{p}_i + \beta_i \mathbf{q}_i) \right] + \left[ v + \sum_{i=1}^m (\alpha_i \mathbf{p}_i - \beta_i \mathbf{q}_i) \right] \quad (\text{II.8})$$

where  $\alpha_i$  and  $\beta_i$  are defined by

$$\begin{aligned} \alpha_i &:= \mathbf{x}^\dagger \mathbf{J}_{2(n+k)} \mathbf{q}_i \\ \beta_i &:= \mathbf{x}^\dagger \mathbf{J}_{2(n+k)} \mathbf{p}_i. \end{aligned} \quad (\text{II.9})$$

The first term of Eq. (II.8) is an element of  $V_m$ , and using Eq. (II.4), we can show that the second term is an element of  $V_m^\perp$ .

Applying a complex version of the skew-symmetric Gram-Schmidt procedure, as described in Theorem 1.1 of ref. [5], we can form a basis of  $V_m^\perp$  such that the basis vectors satisfy Eqs. (II.4) to (II.6). For any nonzero vector  $\mathbf{q}_{m+1} \in V_m^\perp$ , there is exists a vector  $\mathbf{p}_{m+1} \in V_m^\perp$  such that  $\mathbf{q}_{m+1}^\dagger \mathbf{J}_{2(n+k)} \mathbf{p}_{m+1} \neq 0$ , and we can always normalize these vectors such that  $\mathbf{q}_{m+1}^\dagger \mathbf{J}_{2(n+k)} \mathbf{p}_{m+1} = 1$ . Now let  $V_{m+1} = \text{span}(\mathbf{q}_{m+1}, \mathbf{p}_{m+1})$  and  $V_{m+1}^\perp = \{\mathbf{x} : \mathbf{x}^\dagger \mathbf{J}_{2(n+k)} \mathbf{y} = 0 \quad \forall \mathbf{y} \in V_m \cup V_{m+1}\}$ . We then have

$$\mathbb{C}^{2(n+k)} = V_m \oplus V_{m+1} \oplus V_{m+1}^\perp \quad (\text{II.10})$$

Continuing this procedure, we can build a basis for  $V_{m+1}^\perp$ , etc. such that

$$\mathbb{C}^{2(n+k)} = V_m \oplus V_{m+1} \oplus \dots \oplus V_{n+k}. \quad (\text{II.11})$$

The basis of  $V_{m+1} \oplus \dots \oplus V_{n+k}$  constructed in this procedure defines the rows of  $\mathbf{M}_3$  and  $\mathbf{M}_4$ . We note that as in the usual Gram-Schmidt procedure, this basis is not unique. With these matrices in hand, we can construct  $\mathbf{M}$  that satisfies Eq. (II.3) and extends our conjugate symplectic subsystem to a fully conjugate symplectic system.  $\square$

### III. PROOF OF THE OPTICAL DECOMPOSITION (THEOREM 2 OF MAIN TEXT)

The optical decomposition of Theorem 2 in the main text is a direct concatenation of the following two theorems:

1. The conjugate symplectic singular value decomposition (SVD), which expresses any element of  $\text{Sp}^\dagger(2n)$  as a product of elements of  $\text{Sp}^\dagger(2n) \cap U(2n)$  and of a positive, repeating diagonal matrix.
2. The conjugate symplectic Cosine-Sine decomposition (CSD), which expresses any element of  $\text{Sp}^\dagger(2n) \cap U(2n)$  as a product of block matrices representing frequency-dependent beamsplitters and phase shifters.

These two decompositions are proved in the following two sub-sections. In Section III C we briefly comment on the relation between our approach using the conjugate symplectic SVD and the generalized Cartan/“KAK” decomposition from the theory of Lie groups [6, 7].

### A. The conjugate symplectic SVD

**Theorem 6.** *Let  $M \in \text{Sp}^\dagger(2n)$ . Then, there exists  $U, V \in \text{Sp}^\dagger(2n) \cap U(2n)$  and  $D = \text{diag}(e^{r_1}, \dots, e^{r_n})$  with  $(r_1, \dots, r_n) \in \mathbb{R}^n$  such that*

$$M = U \begin{bmatrix} D & \mathbf{0} \\ \mathbf{0} & D^{-1} \end{bmatrix} V \quad (\text{III.1})$$

Theorem 6 means that the usual SVD can be closed in  $\text{Sp}^\dagger(2n)$ , provided that the matrices  $U$  and  $V$  are carefully chosen. There exists proofs of this theorem in the mathematical literature [8] but they do not intuitively follow the general proof of the SVD. Alternatively, Theorem 6 can be equivalently formulated for indefinite unitary matrices, a theorem known as the hyperbolic Cosine-Sine decomposition [7].

We chose to provide a proof below, inspired from [9], whose canvas is similar to the general SVD.

#### 1. Properties of hermitian conjugate symplectic matrices

We first show important results pertaining to hermitian and conjugate symplectic matrices.

**Proposition 2.** *Let  $M \in \text{Sp}^\dagger(2n)$  and hermitian. Therefore 0 is not eigenvalue of  $M$ . Furthermore, by the spectral theorem, its spectrum is real. Let  $\lambda$  an eigenvalue of  $M$  of multiplicity  $m(\lambda)$  and let  $E(\lambda)$  the associated eigenspace. Then,*

1.  $\lambda^{-1}$  is also an eigenvalue of  $M$  with the same multiplicity:  $m(\lambda) = m(\lambda^{-1})$ .
2. For any orthonormal basis  $(\mathbf{x}_1, \dots, \mathbf{x}_{m(\lambda)})$  of  $E(\lambda)$ , define:

$$\forall i \in \{1, \dots, m(\lambda^{-1})\}, \quad \mathbf{y}_i = -\mathbf{J}\mathbf{x}_i \quad (\text{III.2})$$

Then  $(\mathbf{y}_1, \dots, \mathbf{y}_{m(\lambda)})$  is an orthonormal basis of  $E(\lambda^{-1})$ .

3. If  $\lambda \notin \{1, -1\}$ , then  $(\mathbf{x}_1, \dots, \mathbf{x}_{m(\lambda)}, \mathbf{y}_1, \dots, \mathbf{y}_{m(\lambda)})$  verifies,  $\forall i, j \in \{1, \dots, m(\lambda)\}$ :

$$\langle \mathbf{x}_i | \mathbf{x}_j \rangle = \delta_{ij} \quad (\text{III.3})$$

$$\langle \mathbf{y}_i | \mathbf{y}_j \rangle = \delta_{ij} \quad (\text{III.4})$$

$$\langle \mathbf{x}_i | \mathbf{y}_j \rangle = 0 \quad (\text{III.5})$$

$$\langle \mathbf{x}_i | \mathbf{J} | \mathbf{y}_j \rangle = \delta_{ij} \quad (\text{III.6})$$

Eqs. (III.3) to (III.5) mean that the family of vectors  $(\mathbf{x}_1, \dots, \mathbf{x}_{m(\lambda)}, \mathbf{y}_1, \dots, \mathbf{y}_{m(\lambda)})$  is an orthonormal basis of the direct sum space  $E(\lambda) \oplus E(\lambda^{-1})$ . This is only defined when  $\lambda \neq \lambda^{-1}$ , i.e.  $\lambda \notin \{1, -1\}$ .

Crucially, the matrix interpretation is the following: construct the  $2n \times 2m(\lambda)$  matrix  $V$  whose columns are:  $V = [\mathbf{x}_1 \mid \dots \mid \mathbf{x}_{m(\lambda)} \mid \mathbf{y}_1 \mid \dots \mid \mathbf{y}_{m(\lambda)}]$ . Define the  $2m(\lambda) \times 2m(\lambda)$  symplectic form  $J_{2m(\lambda)}$  as blocks of  $m(\lambda) \times m(\lambda)$  matrices:

$$J_{2m(\lambda)} = \begin{bmatrix} \mathbf{0} & \mathbf{1}_{m(\lambda)} \\ -\mathbf{1}_{m(\lambda)} & \mathbf{0} \end{bmatrix} \quad (\text{III.7})$$

with the previous notation that  $J_{2N} = J$ . Then, Eqs. (III.5) and (III.6) are equivalent to  $V$  being rectangular-symplectic:

$$V^\dagger J V = J_{2m(\lambda)} \quad (\text{III.8})$$

Furthermore, Eqs. (III.3) to (III.5) are equivalent to  $V$  being rectangular-unitary:

$$V^\dagger V = \mathbf{1}_{2m} \quad (\text{III.9})$$

Finally, the fact that the columns of  $V$  are orthonormal eigenvectors implies the partial diagonalization of  $M$ :

$$V^\dagger M V = \begin{bmatrix} \lambda \mathbf{1}_{m(\lambda)} & \mathbf{0} \\ \mathbf{0} & \lambda^{-1} \mathbf{1}_{m(\lambda)} \end{bmatrix} \quad (\text{III.10})$$

*Proof of Proposition 2.* To prove the first point, it suffices to prove the second. Let  $(\mathbf{x}_1, \dots, \mathbf{x}_{m(\lambda)})$  an orthonormal basis of  $E(\lambda)$ . Since  $\mathbf{M} \in \text{Sp}^\dagger(2n)$ , for all  $i \in \{1, \dots, m(\lambda)\}$ :

$$\mathbf{M}^\dagger \mathbf{J} \mathbf{M} \mathbf{x}_i = \mathbf{J} \mathbf{x}_i \implies \mathbf{M}^\dagger (-\mathbf{J} \mathbf{x}_i) = \lambda (-\mathbf{J} \mathbf{x}_i) \implies \mathbf{M} \mathbf{y}_i = \lambda \mathbf{y}_i \quad (\text{III.11})$$

where we identified  $\mathbf{y}_i = \mathbf{J} \mathbf{x}_i$  as in Eq. (III.2) and used the hermiticity of  $\mathbf{M}$  on the last inequality. This means that  $\mathbf{y}_i \in E(\lambda^{-1})$ . Furthermore, the family  $(\mathbf{y}_i, \dots, \mathbf{y}_{m(\lambda)})$  is orthonormal, as for any  $i, j \in \{1, \dots, m(\lambda)\}$ :

$$\langle \mathbf{y}_i | \mathbf{y}_j \rangle = \mathbf{y}_i^\dagger \mathbf{y}_j = \mathbf{x}_i^\dagger \mathbf{J}^\dagger \mathbf{J} \mathbf{x}_j = \mathbf{x}_i^\dagger \mathbf{x}_j = \delta_{ij} \quad (\text{III.12})$$

In terms of dimensions, we have shown that  $m(\lambda^{-1}) \geq m(\lambda)$ . Likewise, one could have started with an orthonormal basis  $(\tilde{\mathbf{y}}_1, \dots, \tilde{\mathbf{y}}_{m(\lambda^{-1})})$  of  $E(\lambda^{-1})$  and constructed, for any  $i \in \{1, \dots, m(\lambda^{-1})\}$ :

$$\tilde{\mathbf{x}}_i = -\mathbf{J} \tilde{\mathbf{y}}_i \quad (\text{III.13})$$

A calculation similar to Eq. (III.12) leads to  $(\tilde{\mathbf{x}}_1, \dots, \tilde{\mathbf{x}}_{m(\lambda^{-1})})$  being an orthonormal family of  $E(\lambda)$ . Therefore  $m(\lambda) \geq m(\lambda^{-1})$ . With the above, we have  $m(\lambda) = m(\lambda^{-1})$  and  $(\mathbf{y}_i, \dots, \mathbf{y}_{m(\lambda)})$  is an orthonormal basis of  $E(\lambda^{-1})$ . Points 2 and 1 are proven. Direct calculation shows that point 3 is also true (Eq. (III.5) uses the fact that  $\lambda \neq \lambda^{-1}$  so the eigenspaces  $E(\lambda)$  and  $E(\lambda^{-1})$  are orthogonal, since  $\mathbf{M}$  is hermitian).  $\square$

The following extends the notions of rectangular-symplectic and unitary to different eigenvalues that are not 1 or  $-1$ .

**Proposition 3.** Let  $\mathbf{M} \in \text{Sp}^\dagger(2n)$  and hermitian. Assume that  $\mathbf{M}$  has two eigenvalues  $\lambda_1, \lambda_2$ , both different from 1 and  $-1$ , and such that  $\lambda_2 \notin \{\lambda_1, \lambda_1^{-1}\}$ . Consider  $(\mathbf{x}_1^1, \dots, \mathbf{x}_{m_1}^1)$  an orthogonal basis of  $E(\lambda_1)$ , and  $(\mathbf{x}_1^2, \dots, \mathbf{x}_{m_2}^2)$  an orthogonal basis of  $E(\lambda_2)$  (we have used the shorthand notation  $m_i = m(\lambda_i)$  for the multiplicity). Construct the families  $(\mathbf{y}_1^1, \dots, \mathbf{y}_{m_1}^1)$  and  $(\mathbf{y}_1^2, \dots, \mathbf{y}_{m_2}^2)$  similarly to Eq. (III.2). Define the  $2(m_1 + m_2) \times 2(m_1 + m_2)$  matrix  $\mathbf{V}$  whose columns are

$$\mathbf{V} = [\mathbf{x}_1^1 \mid \dots \mid \mathbf{x}_{m_1}^1 \mid \mathbf{x}_1^2 \mid \dots \mid \mathbf{x}_{m_2}^2 \mid \mathbf{y}_1^1 \mid \dots \mid \mathbf{y}_{m_1}^1 \mid \mathbf{y}_1^2 \mid \dots \mid \mathbf{y}_{m_2}^2] \quad (\text{III.14})$$

Then,  $\mathbf{V}$  is rectangular-symplectic, rectangular-unitary and partially diagonalizes  $\mathbf{M}$ :

$$\mathbf{V}^\dagger \mathbf{J} \mathbf{V} = \mathbf{J}_{2(m_1+m_2)} \quad (\text{III.15})$$

$$\mathbf{V}^\dagger \mathbf{V} = \mathbf{1}_{2(m_1+m_2)} \quad (\text{III.16})$$

$$\mathbf{V}^\dagger \mathbf{M} \mathbf{V} = \begin{bmatrix} \lambda_1 \mathbf{1}_{m(\lambda_1)} & \mathbf{0} & \mathbf{0} & \mathbf{0} \\ \mathbf{0} & \lambda_2 \mathbf{1}_{m(\lambda_2)} & \mathbf{0} & \mathbf{0} \\ \mathbf{0} & \mathbf{0} & \lambda_1^{-1} \mathbf{1}_{m(\lambda_1)} & \mathbf{0} \\ \mathbf{0} & \mathbf{0} & \mathbf{0} & \lambda_2^{-1} \mathbf{1}_{m(\lambda_2)} \end{bmatrix} \quad (\text{III.17})$$

The proof, not shown here for brevity, is very similar to the third point of the previous proposition, using extensively the fact that two distinct eigenspaces of  $\mathbf{M}$  are orthogonal.

It is straightforward to show (by induction) that Proposition 3 can be extended to all the eigenspaces of  $\mathbf{M}$  at once, except  $E(1)$  and  $E(-1)$ . In other words, let  $m$  be the sum of the multiplicities of all the eigenvalues of a hermitian  $\mathbf{M} \in \text{Sp}^\dagger(2n)$  that are not  $\pm 1$ . Then, one can construct a  $2n \times 2m$  matrix  $\mathbf{V}$  using the associated eigenvectors such that

$$\mathbf{V}^\dagger \mathbf{J} \mathbf{V} = \mathbf{J}_{2m} \quad (\text{III.18})$$

$$\mathbf{V}^\dagger \mathbf{V} = \mathbf{1}_{2m} \quad (\text{III.19})$$

$$\mathbf{V}^\dagger \mathbf{M} \mathbf{V} = \mathbf{D}_0 \quad (\text{III.20})$$

where  $\mathbf{D}_0$  is a  $2m \times 2m$  diagonal matrix composed of the eigenvalues of  $\mathbf{M}$ , except  $\pm 1$ , arranged with their multiplicities in a manner similar to Eq. (III.17).

## 2. The spectral theorem for $\text{HPD} \cap \text{Sp}^\dagger(2n)$

**Theorem 7.** Let  $\mathbf{M} \in \text{Sp}^\dagger(2n)$ . We assume that  $\mathbf{M}$  is hermitian positive definite. Then,  $\mathbf{M}$  can be unitarily diagonalized in  $\text{Sp}^\dagger(2n)$ , i.e. there exists  $\mathbf{U} \in \text{Sp}^\dagger(2n) \cap U(2n)$ , a diagonal matrix of strictly positive real numbers  $\tilde{\mathbf{D}} = \text{diag}(\lambda_1, \dots, \lambda_n) > 0$  such that

$$\mathbf{M} = \mathbf{U} \begin{bmatrix} \tilde{\mathbf{D}} & \mathbf{0} \\ \mathbf{0} & \tilde{\mathbf{D}}^{-1} \end{bmatrix} \mathbf{U}^\dagger \quad (\text{III.21})$$

*Proof.* First recall that since  $\mathbf{M}$  is HPD, its spectrum is strictly positive. Furthermore, if 1 is not an eigenvalue, then the reasoning leading to Eqs. (III.18) to (III.20) directly implies that  $m = n$ , and the matrix  $\mathbf{V}$  thus constructed verifies

$$\mathbf{M} = \mathbf{V} \begin{bmatrix} \tilde{\mathbf{D}} & \mathbf{0} \\ \mathbf{0} & \tilde{\mathbf{D}}^{-1} \end{bmatrix} \mathbf{V}^\dagger \quad (\text{III.22})$$

$$\mathbf{V} \in \text{Sp}^\dagger(2n) \cap U(2n) \quad (\text{III.23})$$

The first equality is due to Eq. (III.20) while the second one uses Eqs. (III.18) and (III.19). This concludes the proof in this special case. We now show that this can be adapted in the case where 1 is eigenvalue of  $\mathbf{M}$ . Use again Eqs. (III.18) to (III.20) to construct such a  $2n \times 2m$  matrix  $\mathbf{V}$ . We use the following notation for the columns of  $\mathbf{V}$ :

$$\mathbf{V} = [\mathbf{x}_1 \mid \dots \mid \mathbf{x}_m \mid \mathbf{y}_1 \mid \dots \mid \mathbf{y}_m] \quad (\text{III.24})$$

By summing the multiplicities to the dimension of the full space, we must have  $m(1) = 2(n - m)$  so  $m(1)$  is even. We write  $m' = m(1)/2 \in \mathbb{N}^*$  for simplicity and we consider an orthonormal basis of  $E(1)$ , which we arbitrarily split in two sets of  $m'$  vectors  $(\mathbf{v}_1, \dots, \mathbf{v}_{m'}, \mathbf{w}_1, \dots, \mathbf{w}_{m'})$ . We then extend the  $2n \times 2m$  matrix  $\mathbf{V}$  into a  $2n \times 2n$  matrix  $\mathbf{V}_1$  by appending the previous family of vectors to it at the correct positions:

$$\mathbf{V}_1 = [\mathbf{v}_1 \mid \dots \mid \mathbf{v}_{m'} \mid \mathbf{x}_1 \mid \dots \mid \mathbf{x}_m \mid \mathbf{w}_1 \mid \dots \mid \mathbf{w}_{m'} \mid \mathbf{y}_1 \mid \dots \mid \mathbf{y}_m] \quad (\text{III.25})$$

Since  $E(1)$  is orthogonal to all the other eigenspaces of  $\mathbf{M}$ , we have  $\mathbf{V}_1 \in U(2n)$ . Furthermore, from Eq. (III.18), we also have the block form

$$\mathbf{V}_1^\dagger \mathbf{J} \mathbf{V}_1 = \begin{bmatrix} \mathbf{A} & \mathbf{0} & \mathbf{B} & \mathbf{0} \\ \mathbf{0} & \mathbf{0} & \mathbf{0} & \mathbf{1}_m \\ \mathbf{C} & \mathbf{0} & \mathbf{D} & \mathbf{0} \\ \mathbf{0} & -\mathbf{1}_m & \mathbf{0} & \mathbf{0} \end{bmatrix} \quad (\text{III.26})$$

where each of the  $\mathbf{A}, \mathbf{B}, \mathbf{C}, \mathbf{D}$  is a  $m' \times m'$  matrix. We write  $\mathbf{J}' = \begin{bmatrix} \mathbf{A} & \mathbf{B} \\ \mathbf{C} & \mathbf{D} \end{bmatrix}$ . In order to conclude, we show that  $\mathbf{J}'$  is unitarily similar to  $\mathbf{J}_{2m'}$ .

First, notice that the left-hand side of Eq. (III.26) is antihermitian. This means, since  $\mathbf{J}_{2m}$  is antihermitian, that  $\mathbf{J}'$  is also antihermitian. By the spectral theorem, it is unitarily similar to a diagonal matrix of its eigenvalues. Let us show that  $\mathbf{J}'$  has the same spectrum as  $\mathbf{J}_{2m'}$ .

Looking at the eigenvalues of the left hand side of Eq. (III.26) :  $\mathbf{V}_1^\dagger \mathbf{J} \mathbf{V}_1$  has the same spectrum as  $\mathbf{J}$  (by similarity, since  $\mathbf{V}_1 \in U(2N)$ ), i.e.  $i$  with multiplicity  $N$  and  $-i$  with same multiplicity  $N$ . This implies that the right hand side must have the same spectrum. One can reorder the rows and columns via an orthogonal permutation matrix  $\mathbf{Q}$  so that the right hand side becomes block diagonal:

$$\mathbf{Q}^\dagger \begin{bmatrix} \mathbf{A} & \mathbf{0} & \mathbf{B} & \mathbf{0} \\ \mathbf{0} & \mathbf{0} & \mathbf{0} & \mathbf{1}_m \\ \mathbf{C} & \mathbf{0} & \mathbf{D} & \mathbf{0} \\ \mathbf{0} & -\mathbf{1}_m & \mathbf{0} & \mathbf{0} \end{bmatrix} \mathbf{Q} = \begin{bmatrix} \begin{bmatrix} \mathbf{A} & \mathbf{B} \\ \mathbf{C} & \mathbf{D} \end{bmatrix} & \mathbf{0} \\ \mathbf{0} & \mathbf{J}_{2m} \end{bmatrix} = \begin{bmatrix} \mathbf{J}' & \mathbf{0} \\ \mathbf{0} & \mathbf{J}_{2m} \end{bmatrix} \quad (\text{III.27})$$

For reference, the permutation matrix  $\mathbf{Q}$  is

$$\mathbf{Q} = \begin{bmatrix} \mathbf{1}_{m'} & \mathbf{0} & \mathbf{0} & \mathbf{0} \\ \mathbf{0} & \mathbf{0} & \mathbf{1}_m & \mathbf{0} \\ \mathbf{0} & \mathbf{1}_{m'} & \mathbf{0} & \mathbf{0} \\ \mathbf{0} & \mathbf{0} & \mathbf{0} & \mathbf{1}_m \end{bmatrix} \quad (\text{III.28})$$

By similarity, all the matrices in the equalities above must have the same spectrum. We write  $P_{\mathbf{G}}(X)$  the characteristic polynomial of a matrix  $\mathbf{G}$ . Since the characteristic polynomial of a block diagonal matrix is the product of the characteristic polynomials of each block, we have

$$P_{\mathbf{J}'}(X) = \frac{P_{\mathbf{J}}(X)}{P_{\mathbf{J}_{2m}}(X)} = \frac{(X - i)^N (X + i)^N}{(X - i)^m (X + i)^m} = (X - i)^{m'} (X + i)^{m'} \quad (\text{III.29})$$

In other words,  $\mathbf{J}'$  has the same spectrum as  $\mathbf{J}_{2m'}$ . Since both matrices are diagonalizable, they are unitarily similar: there exists  $\mathbf{W}' \in U(2m')$  such that

$$\mathbf{J}' = \mathbf{W}' \mathbf{J}_{2m'} \mathbf{W}'^\dagger \quad (\text{III.30})$$

We conclude by reordering the vectors in  $\mathbf{V}_1$  to obtain the desired form of Eq. (III.21). Define  $\mathbf{W} = \begin{bmatrix} \mathbf{W}' & \mathbf{0} \\ \mathbf{0} & \mathbf{1}_{2m} \end{bmatrix}$  such that

$$\begin{bmatrix} \mathbf{J}' & \mathbf{0} \\ \mathbf{0} & \mathbf{J}_{2m} \end{bmatrix} = \mathbf{W} \begin{bmatrix} \mathbf{J}_{2m'} & \mathbf{0} \\ \mathbf{0} & \mathbf{J}_{2m} \end{bmatrix} \mathbf{W}^\dagger = \mathbf{W} \mathbf{Q}^\dagger \mathbf{J} \mathbf{Q} \mathbf{W}^\dagger \quad (\text{III.31})$$

Then, Eq. (III.26) becomes with Eq. (III.31):

$$\mathbf{Q}^\dagger \mathbf{V}_1^\dagger \mathbf{J} \mathbf{V}_1 \mathbf{Q} = \mathbf{W} \mathbf{Q}^\dagger \mathbf{J} \mathbf{Q} \mathbf{W}^\dagger \quad (\text{III.32})$$

Define  $\mathbf{U} = \mathbf{V}_1 \mathbf{Q} \mathbf{W} \mathbf{Q}^\dagger$ . As a product of unitary matrices,  $\mathbf{U}$  is unitary. It is also conjugate symplectic due to Eq. (III.32). Finally, by direct calculation, one has

$$\mathbf{M} = \mathbf{U} \begin{bmatrix} \tilde{\mathbf{D}} & \mathbf{0} \\ \mathbf{0} & \tilde{\mathbf{D}}^{-1} \end{bmatrix} \mathbf{U}^\dagger \quad (\text{III.33})$$

owing to the facts that

1.  $\mathbf{V}_1$  diagonalises  $\mathbf{M}$ .
2.  $\mathbf{Q}^\dagger \mathbf{V}_1^\dagger \mathbf{M} \mathbf{V}_1 \mathbf{Q}$  is a diagonal matrix whose first  $2m'$  coefficients on the diagonal are all 1.
3.  $\mathbf{W}$ 's block form implies that it leaves the previous diagonal matrix unchanged:  $\mathbf{W}^\dagger (\mathbf{Q}^\dagger \mathbf{V}_1^\dagger \mathbf{M} \mathbf{V}_1 \mathbf{Q}) \mathbf{W} = \mathbf{Q}^\dagger \mathbf{V}_1^\dagger \mathbf{M} \mathbf{V}_1 \mathbf{Q}$

This concludes the proof of Theorem 7.  $\square$

### 3. Proof of conjugate symplectic SVD

We are finally able to prove the symplectic SVD with a reasoning similar to the proof of the usual SVD [1, 2].

*Proof of Theorem 6.* Let  $\mathbf{M} \in \text{Sp}^\dagger(2n)$ . Since it is invertible and its hermitian conjugate is also symplectic, the matrix  $\mathbf{M}^\dagger \mathbf{M}$  is HPD and conjugate symplectic. Therefore, by the symplectic HPD spectral theorem (Theorem 7), there exists  $\mathbf{V} \in \text{Sp}^\dagger(2n) \cap U(2n)$ , a diagonal matrix of strictly positive real numbers  $\tilde{\mathbf{D}} = \text{diag}(\Sigma_1, \dots, \Sigma_n) > 0$  such that

$$\mathbf{M}^\dagger \mathbf{M} = \mathbf{V} \mathbf{D} \mathbf{V}^\dagger \quad (\text{III.34})$$

where  $\mathbf{D} = \begin{bmatrix} \tilde{\mathbf{D}}^2 & \mathbf{0} \\ \mathbf{0} & \tilde{\mathbf{D}}^{-2} \end{bmatrix} =: \text{diag}(\lambda_1, \dots, \lambda_{2n})$ . Let us construct the matrix

$$\mathbf{U} = \mathbf{M} \mathbf{V} \mathbf{\Sigma} \quad (\text{III.35})$$

where  $\mathbf{\Sigma} = \mathbf{D}^{-1/2} = \begin{bmatrix} \tilde{\mathbf{D}}^{-1} & \mathbf{0} \\ \mathbf{0} & \tilde{\mathbf{D}} \end{bmatrix} > 0$ . Since the right hand side is a product of conjugate symplectic matrices, we have that  $\mathbf{U} \in \text{Sp}^\dagger(2n)$ . Furthermore,  $\mathbf{U}$  is unitary as can be checked by direct computation:

$$\mathbf{U} \mathbf{U}^\dagger = \mathbf{M} \mathbf{V} \mathbf{\Sigma} \mathbf{\Sigma} \mathbf{V}^\dagger \mathbf{M}^\dagger = \mathbf{M} \mathbf{V} \mathbf{D}^{-2} \mathbf{V}^\dagger \mathbf{M}^\dagger = \mathbf{M} \mathbf{M}^{-1} \mathbf{M}^{-\dagger} \mathbf{M}^\dagger = \mathbf{1} \quad (\text{III.36})$$

where we have used the inverse of Eq. (III.34). Isolating  $\mathbf{M}$  in Eq. (III.35), we have thus shown that

$$\mathbf{M} = \mathbf{U} \begin{bmatrix} \tilde{\mathbf{D}} & \mathbf{0} \\ \mathbf{0} & \tilde{\mathbf{D}}^{-1} \end{bmatrix} \mathbf{V}^\dagger \quad (\text{III.37})$$

where  $\mathbf{U}, \mathbf{V} \in \text{Sp}^\dagger(2n) \cap U(2n)$ , which is exactly the symplectic SVD of Theorem 6.  $\square$

## B. The conjugate symplectic CSD

We provide the following cosine-sine decomposition for unitary and conjugate symplectic matrices.

**Theorem 8.** *The set of  $2n \times 2n$  conjugate symplectic matrices which are also unitary is*

$$\mathrm{Sp}^\dagger(2n) \cap U(2n) = \left\{ \begin{bmatrix} \mathbf{V} & \mathbf{0} \\ \mathbf{0} & \mathbf{V} \end{bmatrix} \begin{bmatrix} \mathbf{C} & -\mathbf{S} \\ \mathbf{S} & \mathbf{C} \end{bmatrix} \begin{bmatrix} \mathbf{W} & \mathbf{0} \\ \mathbf{0} & \mathbf{W} \end{bmatrix} \mid \begin{array}{l} \mathbf{V}, \mathbf{W} \in U(n) \\ \mathbf{C} := \mathrm{diag}(\cos \theta_1, \dots, \cos \theta_n) \\ \mathbf{S} := \mathrm{diag}(\sin \theta_1, \dots, \sin \theta_n) \\ (\theta_1, \dots, \theta_n) \in \mathbb{R}^n \end{array} \right\} \quad (\text{III.38})$$

and without loss of generality, one can fix  $n$  phases among the independent matrix coefficients of  $\mathbf{V}$ .

By isomorphism, this result is equivalent to the following cosine-sine decomposition for matrices which are both unitary and indefinite unitary, obtained from the previous theorem by applying the isomorphism from  $\mathrm{Sp}^\dagger(2n)$  to  $U(n, n)$ , defined as  $\mathbf{M} \mapsto \mathbf{P}^\dagger \mathbf{M} \mathbf{P}$ , to each of the three matrices of the decomposition:

**Theorem 9.** *The set of  $2n \times 2n$  indefinite unitary matrices which are also unitary is*

$$U(n, n) \cap U(2n) = \left\{ \begin{bmatrix} \mathbf{V} & \mathbf{0} \\ \mathbf{0} & \mathbf{V} \end{bmatrix} \begin{bmatrix} e^{i\theta} & \mathbf{0} \\ \mathbf{0} & e^{-i\theta} \end{bmatrix} \begin{bmatrix} \mathbf{W} & \mathbf{0} \\ \mathbf{0} & \mathbf{W} \end{bmatrix} \mid \begin{array}{l} \mathbf{V}, \mathbf{W} \in U(n) \\ e^{i\theta} := \mathrm{diag}(e^{i\theta_1}, \dots, e^{i\theta_n}) \\ \theta := (\theta_1, \dots, \theta_n) \in \mathbb{R}^n \end{array} \right\} \quad (\text{III.39})$$

and without loss of generality, one can fix  $n$  phases among the independent matrix coefficients of  $\mathbf{V}$ .

To prove Theorem 9, we first prove a general, block-matrix result on  $U(n, n) \cap U(2n)$ .

**Theorem 10.** *One has the block-matrix characterization*

$$U(n, n) \cap U(2n) = \left\{ \begin{bmatrix} \mathbf{Q}_1 & \mathbf{0} \\ \mathbf{0} & \mathbf{Q}_2 \end{bmatrix} \mid \mathbf{Q}_1, \mathbf{Q}_2 \in U(n) \right\} \quad (\text{III.40})$$

*Proof.* It is straightforward to check that the right hand side is included in  $U(n, n) \cap U(2n)$ . Reciprocally, let  $\mathbf{M} \in U(n, n) \cap U(2n)$  and show that  $\mathbf{M}$  can be written as a block-diagonal of unitary matrices. By definition of  $U(n, n)$ ,  $\mathbf{M} \mathbf{I}_n \mathbf{M}^\dagger = \mathbf{I}_n$  and multiplying on the right by  $\mathbf{M}$  we obtain that  $[\mathbf{M}, \mathbf{I}_n] = \mathbf{0}$ . Write  $\mathbf{M}$  in block form  $\mathbf{M} = \begin{bmatrix} \mathbf{Q}_1 & \mathbf{R} \\ \mathbf{S} & \mathbf{Q}_2 \end{bmatrix}$  with  $\mathbf{Q}_1, \mathbf{Q}_2, \mathbf{R}, \mathbf{S} \in \mathcal{M}_n(\mathbb{C})$  and explicitly compute the commutator. We find that  $\mathbf{R} = \mathbf{S} = \mathbf{0}$ . Thus  $\mathbf{M}$  is block diagonal. Explicitly computing the unitary condition  $\mathbf{M} \mathbf{M}^\dagger = \mathbf{1}$ , we get that  $\mathbf{Q}_1, \mathbf{Q}_2 \in U(n)$  which concludes the proof.  $\square$

*Proof of Theorem 9.* Let us first notice that the right hand side is included in the left hand side. This is due to the fact that  $U(n, n) \cap U(2n)$  is a group (as the intersection of two subgroups of  $GL_n(\mathbb{C})$ ), thus closed under matrix product, and that the three matrices in the right hand side are elements of  $U(n, n) \cap U(2n)$  per Eq. (III.40).

Reciprocally, let  $\mathbf{M} \in U(n, n) \cap U(2n)$ . Using Eq. (III.40), there exists  $\mathbf{Q}_1, \mathbf{Q}_2 \in U(n)$  such that  $\mathbf{M} = \begin{bmatrix} \mathbf{Q}_1 & \mathbf{0} \\ \mathbf{0} & \mathbf{Q}_2 \end{bmatrix}$ . Consider  $\mathbf{Q}_2^\dagger \mathbf{Q}_1 \in U(n)$ . By the spectral theorem for unitary matrices [2], there exists  $\mathbf{W} \in U(n)$  and  $\theta \in \mathbb{R}^n$  such that

$$\mathbf{Q}_2^\dagger \mathbf{Q}_1 = \mathbf{W}^\dagger e^{2i\theta} \mathbf{W} \quad (\text{III.41})$$

Isolating  $\mathbf{Q}_2$

$$\mathbf{Q}_2 = \mathbf{Q}_1 \mathbf{W}^\dagger e^{-2i\theta} \mathbf{W} \quad (\text{III.42})$$

Therefore, we obtain the decomposition

$$\begin{bmatrix} \mathbf{Q}_1 & \mathbf{0} \\ \mathbf{0} & \mathbf{Q}_2 \end{bmatrix} = \begin{bmatrix} \mathbf{Q}_1 \mathbf{W}^\dagger e^{-i\theta} & \mathbf{0} \\ \mathbf{0} & \mathbf{Q}_1 \mathbf{W}^\dagger e^{-i\theta} \end{bmatrix} \begin{bmatrix} e^{i\theta} & \mathbf{0} \\ \mathbf{0} & e^{-i\theta} \end{bmatrix} \begin{bmatrix} \mathbf{W} & \mathbf{0} \\ \mathbf{0} & \mathbf{W} \end{bmatrix} \quad (\text{III.43})$$

which is the right-hand side of Theorem 9 with  $\mathbf{V} := \mathbf{Q}_1 \mathbf{W}^\dagger e^{-i\theta} \in U(n)$ .  $\square$

Thus we have proved both Theorems 8 and 9. The optical decomposition is immediately proven by concatenating both theorems.

### C. Relationship with KAK decomposition

The proofs of this appendix only relied on elementary algebraic matrix properties. We now briefly discuss how the conjugate symplectic, spectral theorem, SVD and CSD can all be seen as applications of the Cartan and “KAK” decompositions [7]. In the following we briefly sketch this relation.

It is known that the conjugate symplectic group is reductive, that is, its Lie algebra can be written in the so-called Cartan form [10] (the direct sum is to be understood at the level of the vector spaces)

$$\mathfrak{sp}^\dagger(2n) = \mathfrak{k} \oplus \mathfrak{p} \quad (\text{III.44})$$

where

$$\mathfrak{k} = \{ \mathbf{J} \mathbf{S}_c \mid \mathbf{S}_c \in \mathcal{M}_{2n}(\mathbb{C}) \text{ hermitian and } [\mathbf{J}, \mathbf{S}_c] = \mathbf{0} \} \quad (\text{III.45})$$

$$\mathfrak{p} = \{ \mathbf{J} \mathbf{S}_a \mid \mathbf{S}_a \in \mathcal{M}_{2n}(\mathbb{C}) \text{ hermitian and } \{ \mathbf{J}, \mathbf{S}_a \} = \mathbf{0} \} \quad (\text{III.46})$$

Note that  $\mathfrak{k}$  is the Lie algebra associated to the Lie group  $K := \mathfrak{Sp}^\dagger(2n) \cap U(2n)$  while the set  $P := \exp(\mathfrak{p})$  is the set of all HPD and conjugate symplectic matrices.

At the group level, the Cartan form implies the so-called Cartan decomposition for  $\mathfrak{Sp}^\dagger(2n)$ :

$$\mathfrak{Sp}^\dagger(2n) = KP. \quad (\text{III.47})$$

We now decompose the elements in  $P$ . The maximal abelian subalgebra  $\mathfrak{a}$  of  $\mathfrak{p}$  is found to be

$$\mathfrak{a} = \left\{ \begin{bmatrix} \mathbf{d} & \mathbf{0} \\ \mathbf{0} & -\mathbf{d} \end{bmatrix} \mid \mathbf{d} = \text{diag}(d_1, \dots, d_n), (d_1, \dots, d_n) \in \mathbb{R}^n \right\} \quad (\text{III.48})$$

Define  $A := \exp(\mathfrak{a})$ , which is the set of all diagonal matrices of the form  $\begin{bmatrix} \mathbf{D} & \mathbf{0} \\ \mathbf{0} & \mathbf{D}^{-1} \end{bmatrix}$ , where  $\mathbf{D}$  is a diagonal matrix with positive diagonal elements. Then, the “KAK” decomposition states that [10]

$$\mathfrak{p} = \bigcup_{K \in K} K \mathfrak{a} K^{-1} \quad (\text{III.49})$$

or equivalently at the group level,

$$P = \bigcup_{K \in K} K A K^{-1} \quad (\text{III.50})$$

which is exactly Theorem 7, the spectral theorem for  $\text{HPD} \cap \mathfrak{Sp}^\dagger(2n)$ . Then, combining Eq. (III.47) with Eq. (III.49) yields Theorem 6, the conjugate symplectic SVD:

$$\mathfrak{Sp}^\dagger(2n) = K A K \quad (\text{III.51})$$

Finally, applying the “KAK” decomposition to the compact group  $K$  yields Theorem 8, the conjugate symplectic CSD.

### IV. RELATION BETWEEN $\mathfrak{Sp}^\dagger(2n)$ AND $\text{Sp}(4n, \mathbb{R})$ (SECTION III C OF MAIN TEXT)

We provide the details of the connection between the conjugate symplectic group on  $n$  modes,  $\mathfrak{Sp}^\dagger(2n)$  and the real symplectic group on  $2n$  modes,  $\text{Sp}(2n, \mathbb{R})$  as claimed in Section III C of main text. We have seen that the frequency-domain quadratures  $(\hat{q}[\omega], \hat{p}[\omega])$  at each frequency  $\omega > 0$  do not define a single harmonic oscillator because they are not themselves hermitian operators (since  $\hat{q}[\omega]^\dagger = \hat{q}[-\omega] \neq \hat{q}[\omega]$ ). The goal here is to show that, in fact, the quadratures  $(\hat{q}[\omega], \hat{p}[\omega])$  describe two independent harmonic oscillators, and therefore allow an isomorphism between  $\mathfrak{Sp}^\dagger(2n)$  and a proper subgroup of  $\text{Sp}(4n, \mathbb{R})$ .

For the rest of this appendix, we fix  $\omega \in \mathbb{R}$ , which we can choose to be positive without loss of generality:  $\omega > 0$ . We also adopt the convention, unless specified otherwise, that the matrices in normal bold font (e.g.  $\mathbf{P}$ ) have size  $2n \times 2n$ , while other notations for matrices (e.g.  $\underline{\mathbf{P}}$  or  $\mathbb{P}$ ), introduced throughout the appendix, have size  $4n \times 4n$ .

### A. A pair of harmonic oscillators for each frequency

In this section we show that linear combinations of frequency-domain quadratures  $(\hat{q}[\omega], \hat{p}[\omega])$  and  $(\hat{q}[-\omega], \hat{p}[-\omega])$  correspond to a pair of harmonic oscillators. To guide the reader through the notations, we first derive this connection in the case of a single spatial mode, then generalize it to the case of a multimode field.

#### 1. Introduction for a single mode $\hat{a}[\omega]$

Let us first consider a single bosonic mode  $\hat{a}[\omega]$ . Recall that the commutation relation is for  $\omega' \in \mathbb{R}$  by  $[\hat{a}[\omega], \hat{a}[\omega']] = 0$  and  $[\hat{a}[\omega], \hat{a}[\omega']^\dagger] = 2\pi\delta[\omega - \omega']$ , but since we work with  $\omega > 0$  while the domain of the map  $\omega \mapsto \hat{a}[\omega]$  is  $\mathbb{R}$ , we need to take care of the mode at the negative frequency  $\hat{a}[-\omega]$ . Notice from the above that  $\hat{a}[\omega]$  and  $\hat{a}[-\omega]$  commute. Define the operators

$$\hat{\mathcal{A}}[\omega] := \frac{\hat{a}[\omega] + \hat{a}[-\omega]}{\sqrt{2}}, \quad \hat{\mathcal{B}}[\omega] := i\frac{\hat{a}[-\omega] - \hat{a}[\omega]}{\sqrt{2}}, \quad \text{i.e.} \quad \hat{a}[\omega] = \frac{\hat{\mathcal{A}}[\omega] + i\hat{\mathcal{B}}[\omega]}{\sqrt{2}}, \quad \hat{a}[-\omega] = \frac{\hat{\mathcal{A}}[\omega] - i\hat{\mathcal{B}}[\omega]}{\sqrt{2}} \quad (\text{IV.1})$$

with the symmetry properties  $\hat{\mathcal{A}}[-\omega] = \hat{\mathcal{A}}[\omega]$ ,  $\hat{\mathcal{B}}[-\omega] = -\hat{\mathcal{B}}[\omega]$ . Crucially, notice that  $\hat{\mathcal{A}}[\omega]$  and  $\hat{\mathcal{B}}[\omega]$  represent two bosonic annihilation operators of two harmonic oscillators: for  $\omega' > 0$ ,

$$[\hat{\mathcal{A}}[\omega], \hat{\mathcal{A}}[\omega']^\dagger] = 2\pi\delta[\omega - \omega'] \quad (\text{IV.2})$$

$$[\hat{\mathcal{B}}[\omega], \hat{\mathcal{B}}[\omega']^\dagger] = 2\pi\delta[\omega - \omega'] \quad (\text{IV.3})$$

$$[\hat{\mathcal{A}}[\omega], \hat{\mathcal{B}}[\omega']^\dagger] = [\hat{\mathcal{A}}[\omega], \hat{\mathcal{B}}[\omega']^\dagger] = 0 \quad (\text{IV.4})$$

We emphasize that these commutation relations are only true when both  $\omega$  and  $\omega'$  have the same sign, here both are positive. Therefore, there is no longer a direct correspondence with their time-domain form, as the Fourier transform requires integrating over both positive and negative frequencies. Nevertheless, we will see in the following how the quadratures associated to these new ladder operators appear in the symplectodyne detection schemes.

One can now naturally define the associated quadrature operators as

$$\hat{q}^{\mathcal{A}}[\omega] := \frac{\hat{\mathcal{A}}[\omega] + \hat{\mathcal{A}}[\omega]^\dagger}{\sqrt{2}}, \quad \hat{p}^{\mathcal{A}}[\omega] := i\frac{\hat{\mathcal{A}}[\omega]^\dagger - \hat{\mathcal{A}}[\omega]}{\sqrt{2}} \quad (\text{IV.5})$$

$$\hat{q}^{\mathcal{B}}[\omega] := \frac{\hat{\mathcal{B}}[\omega] + \hat{\mathcal{B}}[\omega]^\dagger}{\sqrt{2}}, \quad \hat{p}^{\mathcal{B}}[\omega] := i\frac{\hat{\mathcal{B}}[\omega]^\dagger - \hat{\mathcal{B}}[\omega]}{\sqrt{2}} \quad (\text{IV.6})$$

which satisfy  $\hat{q}^{\mathcal{A},\mathcal{B}}[\omega]^\dagger = \hat{q}^{\mathcal{A},\mathcal{B}}[\omega]$ ,  $\hat{p}^{\mathcal{A},\mathcal{B}}[\omega]^\dagger = \hat{p}^{\mathcal{A},\mathcal{B}}[\omega]$  and the corresponding commutation relations, again for  $\omega' > 0$  only:

$$[\hat{q}^{\mathcal{A}}[\omega], \hat{p}^{\mathcal{A}}[\omega']] = [\hat{q}^{\mathcal{B}}[\omega], \hat{p}^{\mathcal{B}}[\omega']] = 2\pi i\delta[\omega - \omega'] \quad (\text{IV.7})$$

$$[\hat{q}^{\mathcal{A}}[\omega], \hat{q}^{\mathcal{B}}[\omega']] = [\hat{q}^{\mathcal{A}}[\omega], \hat{p}^{\mathcal{B}}[\omega']] = 0 \quad (\text{IV.8})$$

Finally, note that these quadratures can be related to the non-hermitian frequency-domain quadratures  $(\hat{q}[\pm\omega], \hat{p}[\pm\omega])$  as

$$\hat{q}[\omega] = \frac{\hat{q}^{\mathcal{A}}[\omega] + i\hat{q}^{\mathcal{B}}[\omega]}{\sqrt{2}}, \quad \hat{p}[\omega] = \frac{\hat{p}^{\mathcal{A}}[\omega] + i\hat{p}^{\mathcal{B}}[\omega]}{\sqrt{2}} \quad (\text{IV.9})$$

or equivalently

$$\hat{q}^{\mathcal{A}}[\omega] = \frac{\hat{q}[\omega] + \hat{q}[\omega]^\dagger}{\sqrt{2}}, \quad \hat{q}^{\mathcal{B}}[\omega] = i\frac{\hat{q}[\omega]^\dagger - \hat{q}[\omega]}{\sqrt{2}} \quad (\text{IV.10})$$

$$\hat{p}^{\mathcal{A}}[\omega] = \frac{\hat{p}[\omega] + \hat{p}[\omega]^\dagger}{\sqrt{2}}, \quad \hat{p}^{\mathcal{B}}[\omega] = i\frac{\hat{p}[\omega]^\dagger - \hat{p}[\omega]}{\sqrt{2}} \quad (\text{IV.11})$$

## 2. General, multimode case: doubled forms

We are now ready to generalize the results of the previous section to the multimode case: consider  $n$  spatial modes  $(\hat{a}_1[\omega], \dots, \hat{a}_n[\omega])$  regrouped in the vector operator  $\hat{\mathbf{a}}[\omega]$  of length  $2n$ . Define the vector operator  $\hat{\mathbf{a}}[\omega]$  of length  $4n$ , the so-called *doubled form* of  $\hat{\mathbf{a}}[\omega]$  as  $\hat{\mathbf{a}}[\omega] = \begin{bmatrix} \hat{\mathbf{a}}[\omega] \\ \hat{\mathbf{a}}[-\omega] \end{bmatrix}$ . To make the ordering explicit,  $\hat{\mathbf{a}}[\omega] = [\hat{a}_1[\omega], \dots, \hat{a}_n[\omega], \hat{a}_1[-\omega]^\dagger, \dots, \hat{a}_n[-\omega]^\dagger, \hat{a}_1[\omega], \dots, \hat{a}_n[\omega], \hat{a}_1[-\omega]^\dagger, \dots, \hat{a}_n[-\omega]^\dagger]^\top$ . It satisfies the commutation relation, for any  $j, k \in \{1, \dots, 4n\}$  and  $\omega' > 0$ :

$$[\hat{\mathbf{a}}_j[\omega], \hat{\mathbf{a}}_k[\omega']^\dagger] = 2\pi\delta[\omega - \omega'] \underline{I}_{jk} \quad (\text{IV.12})$$

with the  $4n \times 4n$  matrix  $\underline{I} := \text{diag}(\mathbf{I}_n, \mathbf{I}_n)$ , the doubled form of the indefinite unitary form  $\mathbf{I}_n$  defined in main text Definition 6.

From  $\hat{\mathbf{a}}[\omega]$ , we can construct the vector operator  $\hat{\mathbf{A}}[\omega] := [\hat{A}_1[\omega], \dots, \hat{A}_n[\omega], \hat{A}_1[\omega]^\dagger, \dots, \hat{A}_n[\omega]^\dagger, \hat{B}_1[\omega], \dots, \hat{B}_n[\omega], \hat{B}_1[\omega]^\dagger, \dots, \hat{B}_n[\omega]^\dagger]^\top$  as

$$\hat{\mathbf{A}}[\omega] = \mathbb{P} \hat{\mathbf{a}}[\omega] \quad (\text{IV.13})$$

where the  $4n \times 4n$  matrix  $\mathbb{P}$  is the analogue of  $\mathbf{P}$  (from main text Eq. (29)) enlarged to  $2n$  modes:  $\mathbb{P} := \frac{1}{\sqrt{2}} \begin{bmatrix} \mathbf{1}_{2n} & \mathbf{1}_{2n} \\ -i\mathbf{1}_{2n} & i\mathbf{1}_{2n} \end{bmatrix} \in U(4n)$ . We naturally obtain the generalization of the commutation relations Eqs. (IV.2) to (IV.4): for any  $j, k \in \{1, \dots, 4n\}$  and  $\omega' > 0$ ,  $[\hat{\mathbf{A}}_j[\omega], \hat{\mathbf{A}}_k[\omega']^\dagger] = 2\pi\delta[\omega - \omega'] \underline{I}_{jk}$ . This can be obtained from Eqs. (IV.12) and (IV.13) by noticing that  $\mathbb{P}\mathbb{P}^\dagger = \underline{I}$ .

From Eq. (IV.13), we can construct the vector operator of quadratures  $\hat{\mathbf{X}}[\omega] := [\hat{q}_1^A[\omega], \dots, \hat{q}_n^A[\omega], \hat{p}_1^A[\omega], \dots, \hat{p}_n^A[\omega], \hat{q}_1^B[\omega], \dots, \hat{q}_n^B[\omega], \hat{p}_1^B[\omega], \dots, \hat{p}_n^B[\omega]]^\top$ , of length  $4n$ , as  $\hat{\mathbf{X}}[\omega] = \underline{\mathbf{P}} \hat{\mathbf{A}}[\omega]$ , where  $\underline{\mathbf{P}} := \text{diag}(\mathbf{P}, \mathbf{P}) \in U(4n) \cap U(2n, 2n)$  (see Eq. (III.40) for the latter inclusion) is the doubled form of  $\mathbf{P}$ . While  $\mathbb{P}$  is different from  $\underline{\mathbf{P}}$ , we note that  $\underline{\mathbf{P}}\underline{\mathbf{P}}^\dagger = \mathbb{P}$ . The analogue of  $\mathbf{P}\mathbf{I}_n\mathbf{P}^\dagger = i\mathbf{J}$  is  $\underline{\mathbf{P}}\underline{\mathbf{I}}\underline{\mathbf{P}}^\dagger = i\underline{\mathbf{J}}$ , where  $\underline{\mathbf{J}} := \text{diag}(\mathbf{J}, \mathbf{J})$ , the doubled form of  $\mathbf{J}$ .

This leads to the CCR on  $\hat{\mathbf{X}}[\omega]$ : for any  $j, k \in \{1, \dots, 4n\}$  and  $\omega' > 0$ ,  $[\hat{\mathbf{X}}_j[\omega], \hat{\mathbf{X}}_k[\omega']^\dagger] = 2\pi i \delta[\omega - \omega'] \underline{J}_{jk}$ . As expected but nonetheless importantly, this CCR equation differs from the one on the frequency-domain quadratures  $\hat{\mathbf{x}}[\omega]$  (main text Eq. (9)) because the operators  $\hat{\mathbf{X}}_j[\omega]$  are hermitian:  $\hat{\mathbf{X}}_j[\omega]^\dagger = \hat{\mathbf{X}}_j[\omega]$ . Thus, at fixed  $\omega > 0$ , the  $4n$ -long vector of quadratures  $\hat{\mathbf{X}}[\omega]$  defines  $2n$  bona fide harmonic oscillators. In the following, we call  $\hat{\mathbf{X}}[\omega]$  the *bona fide quadrature vector operator*.

Akin to Eq. (IV.13), it is possible to relate  $\hat{\mathbf{X}}[\omega]$  to the doubled form of the quadrature vector  $\hat{\mathbf{x}}[\omega]$ , namely  $\hat{\mathbf{x}}[\omega] := [\hat{\mathbf{x}}[\omega], \hat{\mathbf{x}}[-\omega]]^\top$ , through

$$\hat{\mathbf{X}}[\omega] = \mathbb{P} \hat{\mathbf{x}}[\omega] \quad (\text{IV.14})$$

## B. Input and output relations

### 1. Real form of a complex matrix

The analogue of the input-output relation in main text Eq. (19) in doubled form is  $\hat{\mathbf{x}}^{\text{out}}[\omega] = \underline{\mathbf{M}}[\omega] \hat{\mathbf{x}}^{\text{in}}[\omega]$  with the doubled form of the transfer matrix

$$\underline{\mathbf{M}}[\omega] = \text{diag}(\mathbf{M}[\omega], \mathbf{M}^*[\omega]) \quad (\text{IV.15})$$

While the condition  $\mathbf{M}[\omega] \in \text{Sp}^\dagger(2n)$  implies that  $\underline{\mathbf{M}}[\omega] \in \text{Sp}^\dagger(2n) \oplus \text{Sp}^\dagger(2n)$ , the converse is not true in general. Indeed, a matrix  $\underline{\mathbf{A}}$ , belonging in  $\text{Sp}^\dagger(2n) \oplus \text{Sp}^\dagger(2n)$ , has the general form  $\underline{\mathbf{A}} = \text{diag}(\mathbf{B}, \mathbf{C})$  where  $(\mathbf{B}, \mathbf{C}) \in \text{Sp}^\dagger(2n)^2$ , which is not of the form of Eq. (IV.15) since  $\mathbf{B} \neq \mathbf{C}^*$  in general. In fact, the doubled matrix  $\underline{\mathbf{M}}[\omega]$  defined in Eq. (IV.15) contains exactly the same amount of information as the actual transfer matrix  $\mathbf{M}[\omega] \in \text{Sp}^\dagger(2n)$ . Therefore, we write  $\underline{\mathbf{M}}[\omega] \equiv \mathbf{M}[\omega]$ , where the symbol  $\equiv$  is to be understood as an equality in the isomorphic sense of the doubled form. Thus the following definition.

**Definition 3.** The doubled form  $\underline{\text{Sp}}^\dagger(2n)$  of the conjugate symplectic group  $\text{Sp}^\dagger(2n)$  is the set

$$\underline{\text{Sp}}^\dagger(2n) = \left\{ \text{diag}(\mathbf{M}, \mathbf{M}^*) \in GL_{4n}(\mathbb{C}) \mid \mathbf{M} \in \text{Sp}^\dagger(2n) \right\} \quad (\text{IV.16})$$

It is a matrix Lie group, isomorphic to  $\text{Sp}^\dagger(2n)$ .

The previous doubled form transfer function can be translated onto the bona fide quadratures:  $\hat{\mathbf{X}}^{\text{out}}[\omega] = \mathfrak{M}[\omega] \hat{\mathbf{X}}^{\text{in}}[\omega]$  where the bona fide transfer function  $\mathfrak{M}[\omega]$  can be related to  $\underline{\mathbf{M}}[\omega]$  using Eq. (IV.14):

$$\mathfrak{M}[\omega] := \mathbb{P} \underline{\mathbf{M}}[\omega] \mathbb{P}^\dagger = \begin{bmatrix} \text{Re}(\underline{\mathbf{M}}[\omega]) & -\text{Im}(\underline{\mathbf{M}}[\omega]) \\ \text{Im}(\underline{\mathbf{M}}[\omega]) & \text{Re}(\underline{\mathbf{M}}[\omega]) \end{bmatrix} \quad (\text{IV.17})$$

where in this last equality, the notations  $\text{Re}(\cdot)$  and  $\text{Im}(\cdot)$  correspond to element-wise real and imaginary parts, i.e.  $\text{Re}(\underline{\mathbf{M}}) = (\underline{\mathbf{M}} + \underline{\mathbf{M}}^*)/2$  and  $\text{Im}(\underline{\mathbf{M}}) = i(\underline{\mathbf{M}}^* - \underline{\mathbf{M}})/2$ .

Importantly, this last equality is nothing but the real form of the complex matrix  $\underline{\mathbf{M}}[\omega]$ . In particular,  $\mathfrak{M}[\omega]$  is real-valued, which is consistent with the fact that  $\hat{\mathbf{X}}[\omega]$  is hermitian.

Furthermore, since  $\underline{\mathbf{M}}[\omega], \underline{\mathbf{M}}[\omega]^* \in \text{Sp}^\dagger(2n)$ , it is straightforward to check that

$$\mathfrak{M}[\omega] \underline{\mathbf{J}} \mathfrak{M}[\omega]^T = \underline{\mathbf{J}} \quad (\text{IV.18})$$

## 2. Formal approach

To formalize the derivation above, let us define the set of all matrices which satisfy the previous equation. It is clearly isomorphic to  $\text{Sp}(4n, \mathbb{R})$  but for clarity, since  $\underline{\mathbf{J}} \neq \begin{bmatrix} \mathbf{0} & \mathbf{1}_{2n} \\ -\mathbf{1}_{2n} & \mathbf{0} \end{bmatrix}$ , let us use a slightly different notation:

**Definition 4.** The set  $\mathfrak{Sp}(4n, \mathbb{R})$  is

$$\mathfrak{Sp}(4n, \mathbb{R}) := \{ \mathfrak{M} \in \mathcal{M}_{4n}(\mathbb{R}) \mid \mathfrak{M} \underline{\mathbf{J}} \mathfrak{M}^T = \underline{\mathbf{J}} \} \quad (\text{IV.19})$$

It is a matrix Lie group, isomorphic to  $\text{Sp}(4n, \mathbb{R})$  through the linear map

$$\begin{aligned} \mathfrak{Sp}(4n, \mathbb{R}) &\rightarrow \text{Sp}(4n, \mathbb{R}) \\ \mathfrak{M} &\mapsto \mathfrak{Q} \mathfrak{M} \mathfrak{Q} \end{aligned} \quad (\text{IV.20})$$

where the change of basis matrix  $\mathfrak{Q} \in O(4n)$  is defined by  $n \times n$  blocks:

$$\mathfrak{Q} := \begin{bmatrix} \mathbf{1}_n & \mathbf{0} & \mathbf{0} & \mathbf{0} \\ \mathbf{0} & \mathbf{0} & \mathbf{1}_n & \mathbf{0} \\ \mathbf{0} & \mathbf{1}_n & \mathbf{0} & \mathbf{0} \\ \mathbf{0} & \mathbf{0} & \mathbf{0} & \mathbf{1}_n \end{bmatrix} = \mathfrak{Q}^T \quad (\text{IV.21})$$

Let us also define the set of all real forms of a complex (invertible)  $2n \times 2n$  matrix:

**Definition 5.** The set  $\mathfrak{R}(2n)$  is

$$\mathfrak{R}(2n) = \left\{ \begin{bmatrix} \text{Re}(\underline{\mathbf{A}}) & -\text{Im}(\underline{\mathbf{A}}) \\ \text{Im}(\underline{\mathbf{A}}) & \text{Re}(\underline{\mathbf{A}}) \end{bmatrix} \in GL_{4n}(\mathbb{R}) \mid \underline{\mathbf{A}} \in GL_{2n}(\mathbb{C}) \right\} \quad (\text{IV.22})$$

It is a real matrix Lie group, isomorphic to  $GL_{2n}(\mathbb{C})$ . Equivalently, we define its transformation under the change of basis  $\mathfrak{Q}$  as

$$\tilde{\mathfrak{R}}(2n) := \mathfrak{Q} \mathfrak{R}(2n) \mathfrak{Q} = \left\{ \begin{bmatrix} \text{Re}(\underline{\mathbf{A}}_{11}) & -\text{Im}(\underline{\mathbf{A}}_{11}) & \text{Re}(\underline{\mathbf{A}}_{12}) & -\text{Im}(\underline{\mathbf{A}}_{12}) \\ \text{Im}(\underline{\mathbf{A}}_{11}) & \text{Re}(\underline{\mathbf{A}}_{11}) & \text{Im}(\underline{\mathbf{A}}_{12}) & \text{Re}(\underline{\mathbf{A}}_{12}) \\ \text{Re}(\underline{\mathbf{A}}_{21}) & -\text{Im}(\underline{\mathbf{A}}_{21}) & \text{Re}(\underline{\mathbf{A}}_{22}) & -\text{Im}(\underline{\mathbf{A}}_{22}) \\ \text{Im}(\underline{\mathbf{A}}_{21}) & \text{Re}(\underline{\mathbf{A}}_{21}) & \text{Im}(\underline{\mathbf{A}}_{22}) & \text{Re}(\underline{\mathbf{A}}_{22}) \end{bmatrix} \in GL_{4n}(\mathbb{R}) \mid \begin{bmatrix} \underline{\mathbf{A}}_{11} & \underline{\mathbf{A}}_{12} \\ \underline{\mathbf{A}}_{21} & \underline{\mathbf{A}}_{22} \end{bmatrix} \in GL_{2n}(\mathbb{C}) \right\} \quad (\text{IV.23})$$

From the previous Eqs. (IV.17) and (IV.18), we have effectively established an isomorphism between  $\text{Sp}^\dagger(2n)$  and  $\mathfrak{Sp}(4n, \mathbb{R}) \cap \mathfrak{R}(2n)$  or  $\text{Sp}(4n, \mathbb{R}) \cap \tilde{\mathfrak{R}}(2n)$ :

$$\text{Sp}^\dagger(2n) \cong \mathfrak{Sp}(4n, \mathbb{R}) \cap \mathfrak{R}(2n) \cong \text{Sp}(4n, \mathbb{R}) \cap \tilde{\mathfrak{R}}(2n) \quad (\text{IV.24})$$

### C. Physical interpretation of $\text{Sp}^\dagger(2n) \neq \mathfrak{Sp}(4n, \mathbb{R})$

Looking back at the definition of  $\hat{\mathfrak{X}}[\omega]$  as a vector of  $2n$  pairs of bona-fide quadratures, it may be tempting to conclude that the conjugate symplectic formalism on the  $n$  modes is equivalent to working with  $2n$  modes, but keeping the real symplectic structure of the transfer matrices. In other words, do we have  $\mathbf{M}[\omega] \in \text{Sp}^\dagger(2n) \stackrel{?}{\iff} \mathfrak{M}[\omega] \in \mathfrak{Sp}(4n, \mathbb{R})$ ? As we have mathematically shown in the previous section, this assumption is false. In this section, we provide some physical insight as to what the transformations in  $\mathfrak{Sp}(4n, \mathbb{R})$  represent.

Let us consider a general element  $\mathfrak{M}'[\omega]$  of  $\mathfrak{Sp}(4n, \mathbb{R})$  and let us examine what kind of transformation this represents in the hypothesis that  $\mathfrak{M}'[\omega] \notin \mathfrak{R}(2n)$ . Using the transformation Eq. (IV.17), a direct block matrix computation shows that the corresponding matrix  $\mathbf{M}'[\omega] := \mathbb{P}^\dagger \mathfrak{M}'[\omega] \mathbb{P}$  has the  $2n \times 2n$  block matrix form

$$\mathbf{M}'[\omega] = \begin{bmatrix} \mathbf{F}[\omega] & \mathbf{G}[\omega] \\ \mathbf{G}^*[\omega] & \mathbf{F}^*[\omega] \end{bmatrix} \quad (\text{IV.25})$$

where  $\mathbf{F}$  and  $\mathbf{G}$  are  $2n \times 2n$  complex valued-matrices which are linear combinations of the matrix elements in  $\mathfrak{M}'[\omega]$ . As we have previously seen, this is compatible with the doubled form of Eq. (IV.15) if and only if  $\mathfrak{M}'[\omega] \in \mathfrak{R}(2n)$ , which implies  $\mathbf{G}[\omega] = \mathbf{0}$ . Conversely,  $\mathfrak{M}'[\omega] \notin \mathfrak{R}(2n)$  if and only if  $\mathbf{G}[\omega] \neq \mathbf{0}$ . In this case, we can consider some non-zero element  $G_{jk}[\omega]$  and solely focus on the classical transfer function from input  $k$  to output  $j$ , all other inputs taken to be zero. Recall that the definition of the doubled form is

$$\begin{bmatrix} \hat{\mathbf{x}}^{\text{out}}[\omega] \\ \hat{\mathbf{x}}^{\text{out}}[-\omega] \end{bmatrix} = \begin{bmatrix} \mathbf{F}[\omega] & \mathbf{G}[\omega] \\ \mathbf{G}^*[\omega] & \mathbf{F}^*[\omega] \end{bmatrix} \begin{bmatrix} \hat{\mathbf{x}}^{\text{in}}[\omega] \\ \hat{\mathbf{x}}^{\text{in}}[-\omega] \end{bmatrix} \quad (\text{IV.26})$$

Therefore,  $x_j^{\text{out}}[\omega] = F_{jk}[\omega]x_k^{\text{in}}[\omega] + G_{jk}[\omega]x_k^{\text{in}}[-\omega]$  and notice that this is not time-invariant as its time-domain transfer function involves the time-reversal operator:

$$x_j^{\text{out}}(t) = \int_{-\infty}^{+\infty} F_{jk}(\tau)x_k^{\text{in}}(t-\tau) + G_{jk}(\tau)x_k^{\text{in}}(-(t-\tau)) d\tau \quad (\text{IV.27})$$

In conclusion, we have shown that general real-symplectic transformations between the bona fide quadratures contradict the hypothesis of a time-invariant input-output relation.

### D. Physical detectability of the bona fide quadratures $\hat{\mathfrak{X}}[\omega]$

Let us return to the case of an LTI system, i.e.  $\mathbf{G} = \mathbf{0}$ . We study in this section the measurability of the bona fide quadratures under the detection schemes described in the main text.

#### 1. Synodyne measurement of the bona fide quadratures

We show here that the bona fide quadrature vector  $\hat{\mathfrak{X}}[\omega]$  can be physically measured through synodyne detection. We focus on the single-mode case.

Recall that synodyne detection consists in modulating the local oscillator such that the resulting photocurrent at zero frequency is (see Section V A of main text):

$$\hat{I}[0] = \frac{1}{\sqrt{2}} \left( \alpha_{q0}^{\text{SD}*} \hat{q}[\omega_0] + \alpha_{q0}^{\text{SD}} \hat{q}[-\omega_0] + \alpha_{p0}^{\text{SD}*} \hat{p}[\omega_0] + \alpha_{p0}^{\text{SD}} \hat{p}[-\omega_0] \right) \quad (\text{IV.28})$$

where  $(\alpha_{q0}^{\text{SD}}, \alpha_{p0}^{\text{SD}}) \in \mathbb{C}^2$  encode four independent, real-valued degrees of freedom. Expressing this as a function of the bona fide quadratures yields

$$\hat{I}[0] = \text{Re}(\alpha_{q0}^{\text{SD}}) \hat{q}^{\mathcal{A}}[\omega_0] + \text{Re}(\alpha_{p0}^{\text{SD}}) \hat{p}^{\mathcal{A}}[\omega_0] + \text{Im}(\alpha_{q0}^{\text{SD}}) \hat{q}^{\mathcal{B}}[\omega_0] + \text{Im}(\alpha_{p0}^{\text{SD}}) \hat{p}^{\mathcal{B}}[\omega_0] \quad (\text{IV.29})$$

We thus see that by tuning the amplitude and phase of the synodyne modulation  $(\alpha_{q0}^{\text{SD}}, \alpha_{p0}^{\text{SD}})$ , we are able to measure any linear combination of the bona fide quadrature vector, thus confirming that they are indeed physical quantities.

## 2. Spectral correlations of the bona fide quadratures

We determine here the relationship between the SDM of the bona fide quadratures  $\bar{\mathbf{S}}^{\mathbf{x}}[\omega]$  and the SDM  $\bar{\mathbf{S}}[\omega]$  of the two-photon quadratures.  $\bar{\mathbf{S}}^{\mathbf{x}}[\omega]$  is defined for  $\omega > 0$  by its matrix elements  $\ell, m \in \{1, \dots, 4n\}$  as

$$\bar{S}_{\ell m}^{\mathbf{x}}[\omega] = \frac{1}{4\pi\delta[0]} \left\langle \left\{ \hat{\mathbf{x}}_{\ell}[\omega], \hat{\mathbf{x}}_m[\omega]^{\dagger} \right\} \right\rangle = \frac{1}{4\pi\delta[0]} \left\langle \left\{ \hat{\mathbf{x}}_{\ell}[\omega], \hat{\mathbf{x}}_m[\omega] \right\} \right\rangle \quad (\text{IV.30})$$

Following a calculation similar to Section IV B, we find that

$$\bar{\mathbf{S}}^{\mathbf{x}}[\omega] = \begin{bmatrix} \text{Re}(\bar{\mathbf{S}}[\omega]) & -\text{Im}(\bar{\mathbf{S}}[\omega]) \\ \text{Im}(\bar{\mathbf{S}}[\omega]) & \text{Re}(\bar{\mathbf{S}}[\omega]) \end{bmatrix} \quad (\text{IV.31})$$

To interpret this block form, let us write  $\bar{\mathbf{S}}^{\mathbf{x}}[\omega]$  in block form as

$$\bar{\mathbf{S}}^{\mathbf{x}}[\omega] = \begin{bmatrix} \bar{\mathbf{S}}^{\mathcal{AA}}[\omega] & \bar{\mathbf{S}}^{\mathcal{AB}}[\omega] \\ \bar{\mathbf{S}}^{\mathcal{BA}}[\omega] & \bar{\mathbf{S}}^{\mathcal{BB}}[\omega] \end{bmatrix} \quad (\text{IV.32})$$

where, for any  $j, k \in \{1, \dots, 2n\}$ ,

$$\bar{S}_{jk}^{\mathcal{AA}}[\omega] = \frac{1}{4\pi\delta[0]} \left\langle \left\{ \hat{x}_j^{\mathcal{A}}[\omega], \hat{x}_k^{\mathcal{A}}[\omega]^{\dagger} \right\} \right\rangle, \quad \bar{S}_{jk}^{\mathcal{AB}}[\omega] = \frac{1}{4\pi\delta[0]} \left\langle \left\{ \hat{x}_j^{\mathcal{A}}[\omega], \hat{x}_k^{\mathcal{B}}[\omega]^{\dagger} \right\} \right\rangle \quad (\text{IV.33})$$

and similarly for  $\bar{\mathbf{S}}^{\mathcal{BA}}$  and  $\bar{\mathbf{S}}^{\mathcal{BB}}$ . We therefore see that under the LTI hypothesis, the  $\mathcal{A}$  and  $\mathcal{B}$ -quadratures must have the same SDM  $\bar{\mathbf{S}}^{\mathcal{AA}} = \bar{\mathbf{S}}^{\mathcal{BB}} = \text{Re}(\bar{\mathbf{S}}[\omega])$ , and that complex squeezing, which affects the imaginary part of the SDM, appears in entanglement between the two sets of bona fide quadratures:  $\bar{\mathbf{S}}^{\mathcal{AB}}[\omega] = -\text{Im}(\bar{\mathbf{S}}[\omega])$ .

## V. PROOF OF THE UNCERTAINTY PRINCIPLE (THEOREM 3 OF MAIN TEXT) AND CONSEQUENCES

In this section we prove Theorem 3 in the main text and the consequence that the SDM is HPD at all frequencies.

**Theorem.** *Let  $\bar{\mathbf{S}}[\omega]$  be the SDM of  $n$  weak-stationary quantum noises. For any  $\omega \in \mathbb{R}$ , the matrix  $\bar{\mathbf{S}}[\omega] + \mathbf{i}\mathbf{J}/2$  is hermitian, positive semi-definite, i.e.*

$$\bar{\mathbf{S}}[\omega] + \frac{\mathbf{i}}{2}\mathbf{J} \geq 0. \quad (\text{V.1})$$

*Proof.* Since  $\bar{\mathbf{S}}[\omega]$  is hermitian,  $\bar{\mathbf{S}}[\omega] + \frac{\mathbf{i}}{2}\mathbf{J}$  is also hermitian. Let  $\boldsymbol{\alpha} = [\alpha_1, \dots, \alpha_{2N}]^T \in \mathbb{C}^{2N}$  and  $\hat{A}[\omega] = \boldsymbol{\alpha}_j^* \hat{r}_j[\omega]$ . Then, using the CCR relations,

$$\boldsymbol{\alpha}^{\dagger} \left( \bar{\mathbf{S}}[\omega] + \frac{\mathbf{i}}{2}\mathbf{J} \right) \boldsymbol{\alpha} = \frac{\alpha_j^* \alpha_k}{4\pi\delta[0]} \left\langle \left\{ \hat{r}_j[\omega], \hat{r}_k[\omega]^{\dagger} \right\} + [\hat{r}_j[\omega], \hat{r}_k[\omega]^{\dagger}] \right\rangle = \frac{1}{2\pi\delta[0]} \langle \hat{A}[\omega] \hat{A}[\omega]^{\dagger} \rangle = \bar{S}_{AA}[\omega] \geq 0 \quad (\text{V.2})$$

□

We have already seen in Theorem 7 in the main text Appendix A that the SDM is HPD by construction. We will now show that, due to the uncertainty principle (main text Theorem 3), the SDM is actually non-singular; thus the SDM is hermitian positive-definite (HPD).

**Proposition 4.** *Let  $\bar{\mathbf{S}}$  be the SDM of a  $n$ -mode quantum system. For any frequency  $\omega \in \mathbb{R}$ ,  $\bar{\mathbf{S}}[\omega]$  is positive definite.*

*Proof.* We fix a frequency  $\omega \in \mathbb{R}$ . Notice that, because  $\bar{\mathbf{S}}[-\omega] = \bar{\mathbf{S}}[\omega]^*$ , the uncertainty principle yields that  $\bar{\mathbf{S}}[\omega]^* + \mathbf{i}\mathbf{J}/2$  is HPD. We now drop the dependency on  $\omega$  for simplicity. By contradiction, assume that 0 is an eigenvalue of  $\bar{\mathbf{S}}$ . There exists  $\boldsymbol{\alpha} \in \mathbb{C}^{2n} \setminus \{0\}$  such that  $\bar{\mathbf{S}} \boldsymbol{\alpha} = 0$ . Notice that  $\bar{\mathbf{S}}^* \boldsymbol{\alpha}^* = 0$  so 0 is also an eigenvalue of  $\bar{\mathbf{S}}^*$ . Let  $k = \boldsymbol{\alpha}^{\dagger} (\mathbf{i}\mathbf{J}) \boldsymbol{\alpha}$ , which is real since  $(\mathbf{i}\mathbf{J})$  is hermitian. Consider the following cases:

1. Assume  $k > 0$ . Then, from the uncertainty principle,  $\boldsymbol{\alpha}^{*\dagger} \left( \bar{\mathbf{S}}^* + \mathbf{i}\frac{\mathbf{J}}{2} \right) \boldsymbol{\alpha}^* \geq 0$ . Therefore  $-k = \boldsymbol{\alpha}^{*\dagger} \mathbf{i}\mathbf{J} \boldsymbol{\alpha}^* \geq 0$  which constitutes a contradiction.

2. Assume  $k < 0$ . Similarly, from the uncertainty principle,  $\alpha^\dagger (\bar{\mathbf{S}} + i\frac{\mathbf{J}}{2}) \alpha \geq 0$  which results in the contradiction that  $k \geq 0$ .
3. Assume  $k = 0$ . Let  $\epsilon \in \mathbb{R}$  and  $\beta := (\mathbf{1} + i\epsilon\mathbf{J})\alpha$ . Then, a direct computation yields  $\beta^\dagger (\bar{\mathbf{S}} + i\frac{\mathbf{J}}{2}) \beta = \epsilon + \epsilon^2(i\mathbf{J}\alpha)^\dagger \bar{\mathbf{S}}(i\mathbf{J}\alpha)$ . Since  $(i\mathbf{J}\alpha)^\dagger \bar{\mathbf{S}}(i\mathbf{J}\alpha) \geq 0$ , it is always possible to choose a particular  $\epsilon < 0$  such that the right hand side is strictly negative, which contradicts the uncertainty principle.

□

## VI. PROOF OF THE CONJUGATE SYMPLECTIC REDUCTION OF THE SDM (THEOREM 4 OF MAIN TEXT)

In this section we prove Theorem 4 of the main text, which is the conjugate symplectic generalization of Williamson's theorem:

**Theorem 11** (Williamson [11]). *Let  $\mathbf{V}$  a  $2n \times 2n$ , real valued, symmetric, positive definite (SPD) matrix. There exists  $\mathbf{S} \in \text{Sp}(2n, \mathbb{R})$  and a positive diagonal matrix  $\mathbf{\Sigma} = \text{diag}(\Sigma_1, \dots, \Sigma_n) > 0$  such that*

$$\mathbf{V} = \mathbf{S} \begin{bmatrix} \mathbf{\Sigma} & \mathbf{0} \\ \mathbf{0} & \mathbf{\Sigma} \end{bmatrix} \mathbf{S}^T \quad (\text{VI.1})$$

and the  $\Sigma_1, \dots, \Sigma_n$  can be computed as the absolute values of the eigenvalues of the matrix  $i\mathbf{J}\mathbf{V}$ . Furthermore, if  $\mathbf{V}$  satisfies the uncertainty principle,  $\mathbf{V} + i\mathbf{J}/2 \geq 0$ , then for any  $j \in \{1, \dots, n\}$ ,  $\Sigma_j \geq 1/2$ .

In the following we first prove the symplectic reduction for any hermitian positive definite matrix (Theorem 12), then specialize it to the case of a physical SDM, which additionally needs to satisfy the uncertainty principle  $\bar{\mathbf{S}} + i\mathbf{J}/2 \geq 0$ .

### A. Conjugate symplectic reduction for a hermitian positive definite matrix

**Theorem 12.** *Let  $\bar{\mathbf{S}}$  be a  $2n \times 2n$ , complex-valued, hermitian, positive definite (HPD) matrix. There exists*

- $\mathbf{M} \in \text{Sp}^\dagger(2n)$ ;
- a positive diagonal matrix  $\mathbf{\Sigma} = \text{diag}(\Sigma_1, \dots, \Sigma_n)$ ;
- a real matrix  $\mathbf{\Delta} = \text{diag}(\Delta_1, \dots, \Delta_n)$

such that

$$\bar{\mathbf{S}} = \mathbf{M} \begin{bmatrix} \mathbf{\Sigma} & i\mathbf{\Delta} \\ -i\mathbf{\Delta} & \mathbf{\Sigma} \end{bmatrix} \mathbf{M}^\dagger \quad (\text{VI.2})$$

and the  $\Sigma_1, \dots, \Sigma_n$  and  $\Delta_1, \dots, \Delta_n$  can be computed in the following way: the matrix  $i\mathbf{J}\bar{\mathbf{S}}$  has  $n$  real positive eigenvalues (counting their multiplicities)  $\mu_1 \geq \dots \geq \mu_n > 0$  and  $n$  real negative eigenvalues (counting their multiplicities)  $0 > \mu_{n+1} \geq \dots \geq \mu_{2n}$ ; define, for any  $j$  in  $\{1, \dots, n\}$ ,

$$\Sigma_j = \frac{\mu_j - \mu_{n+j}}{2} > 0, \quad \Delta_j = \frac{\mu_j + \mu_{n+j}}{2} \quad (\text{VI.3})$$

Its proof relies on the following lemma.

**Lemma 1** (Indefinite spectral theorem). *Let  $\bar{\mathbf{S}}$  be a  $2n \times 2n$ , complex-valued, hermitian, positive definite (HPD) matrix. There exists  $\mathbf{W} \in U(n, n)$  and a positive diagonal matrix  $\mathbf{D} = \text{diag}(\lambda_1, \dots, \lambda_{2n}) > 0$  such that*

$$\bar{\mathbf{S}} = \mathbf{W} \mathbf{D} \mathbf{W}^\dagger \quad (\text{VI.4})$$

The diagonal elements of  $\mathbf{D}$  are the absolute values of the eigenvalues of  $\mathbf{I}_n \bar{\mathbf{S}}$ , which has  $n$  (counting multiplicities) real positive eigenvalues  $\mu_1 \geq \dots \geq \mu_n > 0$  and  $n$  (counting multiplicities) real negative eigenvalues  $0 > \mu_{n+1} \geq \dots \geq \mu_{2n}$ . One can choose the  $\lambda_j$  such that  $(\lambda_1, \dots, \lambda_n) = (\mu_1, \dots, \mu_n)$  and  $(\lambda_{n+1}, \dots, \lambda_{2n}) = (-\mu_{n+1}, \dots, -\mu_{2n})$ .

*Proof of the lemma.* Let  $\bar{\mathbf{S}}$  a  $2n \times 2n$  HPD matrix. Consider  $\mathbf{A} := \bar{\mathbf{S}}^{1/2} \mathbf{I}_n \bar{\mathbf{S}}^{1/2}$  (recall that  $\mathbf{I}_n$  was defined in Definition 6). Notice that  $\mathbf{A}$  is hermitian so by the spectral theorem there exists  $\mathbf{U} \in U(2n)$  and a real  $2n \times 2n$  diagonal matrix  $\mathbf{\Lambda}$  such that

$$\mathbf{U}^\dagger \mathbf{A} \mathbf{U} = \mathbf{U}^\dagger \bar{\mathbf{S}}^{1/2} \mathbf{I}_n \bar{\mathbf{S}}^{1/2} \mathbf{U} = \mathbf{\Lambda} \quad (\text{VI.5})$$

We now use Sylvester's law of inertia for hermitian matrices (Theorem 1), since, from the above,  $\mathbf{I}_n$  is congruent to  $\mathbf{\Lambda}$  through the invertible matrix  $\bar{\mathbf{S}}^{1/2} \mathbf{U}$ . This implies that  $\mathbf{\Lambda}$  has  $n$  positive and  $n$  negative eigenvalues, which can be ordered such that  $\mathbf{\Lambda} = \text{diag}(\mu_1, \dots, \mu_{2n})$  with  $\mu_1 \geq \dots \geq \mu_n > 0 > \mu_{n+1} \geq \dots \geq \mu_{2n}$ . Then, defining  $\mathbf{D} = |\mathbf{\Lambda}| = \text{diag}(|\mu_1|, \dots, |\mu_{2n}|)$ , a positive diagonal matrix, notice that

$$\mathbf{\Lambda} = \mathbf{D} \mathbf{I}_n = \mathbf{D}^{1/2} \mathbf{I}_n \mathbf{D}^{1/2} \quad (\text{VI.6})$$

Injecting this into Eq. (VI.5) one obtains

$$\mathbf{U}^\dagger \bar{\mathbf{S}}^{1/2} \mathbf{I}_n \bar{\mathbf{S}}^{1/2} \mathbf{U} = \mathbf{D}^{1/2} \mathbf{I}_n \mathbf{D}^{1/2} = \mathbf{D} \mathbf{I}_n \quad (\text{VI.7})$$

We can give a straightforward interpretation of the coefficients of  $\mathbf{D}$ . The four matrices  $\mathbf{\Lambda}$ ,  $\mathbf{A}$ ,  $\mathbf{I}_n \bar{\mathbf{S}}$  and  $\bar{\mathbf{S}} \mathbf{I}_n$  are all similar since

$$\mathbf{U} \mathbf{\Lambda} \mathbf{U}^\dagger = \mathbf{A} = \bar{\mathbf{S}}^{1/2} \mathbf{I}_n \bar{\mathbf{S}}^{1/2} = \bar{\mathbf{S}}^{1/2} (\mathbf{I}_n \bar{\mathbf{S}}) \bar{\mathbf{S}}^{-1/2} \quad (\text{VI.8})$$

$$= \bar{\mathbf{S}}^{-1/2} (\bar{\mathbf{S}} \mathbf{I}_n) \bar{\mathbf{S}}^{1/2} \quad (\text{VI.9})$$

which means that they all have the same spectra. Recalling that  $\mathbf{\Lambda}$  was obtained from the spectral theorem applied to  $\mathbf{A}$ , we deduce that the diagonal terms in  $\mathbf{D}$  are the absolute values of the eigenvalues of  $\mathbf{I}_n \bar{\mathbf{S}}$  (or  $\bar{\mathbf{S}} \mathbf{I}_n$ ).

Taking the inverse of Eq. (VI.7), multiplying on the left by  $\bar{\mathbf{S}}^{1/2} \mathbf{U}$  and on the right by  $\mathbf{U}^\dagger \bar{\mathbf{S}}^{1/2}$  (with  $\mathbf{I}_n^{-1} = \mathbf{I}_n$ ):

$$\mathbf{I}_n = \bar{\mathbf{S}}^{1/2} \mathbf{U} \mathbf{D}^{-1/2} \mathbf{I}_n \mathbf{D}^{-1/2} \mathbf{U}^\dagger \bar{\mathbf{S}}^{1/2} \quad (\text{VI.10})$$

Therefore, let  $\mathbf{W} := \bar{\mathbf{S}}^{1/2} \mathbf{U} \mathbf{D}^{-1/2}$ . From the previous equation we see that  $\mathbf{W} \in U(n, n)$ , and a direct computation yields the desired result in Eq. (VI.4).  $\square$

*Proof of Theorem 12.* Let  $\bar{\mathbf{S}}$  be a  $2n \times 2n$  HPD matrix. Define the matrix  $\mathbf{A} := \mathbf{P}^\dagger \bar{\mathbf{S}} \mathbf{P}$ , with  $\mathbf{P}$  defined in Eq. (29). Notice that  $\mathbf{A}$  is HPD. Applying Lemma 1 to  $\mathbf{A}$ , there exists a  $\mathbf{W} \in U(n, n)$  and  $\mathbf{D} = \text{diag}(\lambda_1, \dots, \lambda_{2n}) > 0$  such that

$$\mathbf{A} = \mathbf{P}^\dagger \bar{\mathbf{S}} \mathbf{P} = \mathbf{W} \mathbf{D} \mathbf{W}^\dagger \quad (\text{VI.11})$$

and we choose the ordering  $(\lambda_1, \dots, \lambda_n) = (\mu_1, \dots, \mu_n)$  and  $(\lambda_{n+1}, \dots, \lambda_{2n}) = (-\mu_{n+1}, \dots, -\mu_{2n})$  where the  $n$  real positive eigenvalues of  $\mathbf{I}_n \mathbf{A}$  are  $(\mu_1, \dots, \mu_n)$  and  $(\mu_{n+1}, \dots, \mu_{2n})$  its  $n$  real negative eigenvalues.

We show that the  $\mu_j$  are also the eigenvalues of the matrix  $\mathbf{i} \mathbf{J} \bar{\mathbf{S}}$ . This can be seen by similarity, as

$$\mathbf{I}_n \mathbf{A} = \mathbf{I}_n \mathbf{P}^\dagger \bar{\mathbf{S}} \mathbf{P} = \mathbf{P}^\dagger \times (\mathbf{i} \mathbf{J} \bar{\mathbf{S}}) \times \mathbf{P} \quad (\text{VI.12})$$

where we used  $\mathbf{P} \mathbf{I}_n \mathbf{P}^\dagger = \mathbf{i} \mathbf{J}$  for the last equality. Thus  $\mathbf{I}_n \mathbf{A}$  and  $\mathbf{i} \mathbf{J} \bar{\mathbf{S}}$  share the same eigenvalues  $\mu_j$ .

We finish the proof by constructing the required form of Theorem 12. Through the group isomorphism  $\text{Sp}^\dagger(2n) \cong U(n, n)$ , the matrix  $\mathbf{M} := \mathbf{P} \mathbf{W} \mathbf{P}^\dagger$  is conjugate symplectic. Furthermore, define the two  $n \times n$  real positive diagonal matrices  $\mathbf{D}_1 = \text{diag}(\lambda_1, \dots, \lambda_n)$  and  $\mathbf{D}_2 = \text{diag}(\lambda_{n+1}, \dots, \lambda_{2n})$  such that  $\mathbf{D} := \text{diag}(\mathbf{D}_1, \mathbf{D}_2)$ . Putting everything into Eq. (VI.11):

$$\mathbf{P}^\dagger \bar{\mathbf{S}} \mathbf{P} = \mathbf{P}^\dagger \mathbf{M} \mathbf{P} \begin{bmatrix} \mathbf{D}_1 & \mathbf{0} \\ \mathbf{0} & \mathbf{D}_2 \end{bmatrix} \mathbf{P}^\dagger \mathbf{M}^\dagger \mathbf{P} \quad (\text{VI.13})$$

so

$$\bar{\mathbf{S}} = \mathbf{M} \mathbf{P} \begin{bmatrix} \mathbf{D}_1 & \mathbf{0} \\ \mathbf{0} & \mathbf{D}_2 \end{bmatrix} \mathbf{P}^\dagger \mathbf{M}^\dagger \quad (\text{VI.14})$$

Explicitly, one finds

$$\mathbf{P} \begin{bmatrix} \mathbf{D}_1 & \mathbf{0} \\ \mathbf{0} & \mathbf{D}_2 \end{bmatrix} \mathbf{P}^\dagger = \frac{1}{2} \begin{bmatrix} \mathbf{D}_1 + \mathbf{D}_2 & i(\mathbf{D}_1 - \mathbf{D}_2) \\ -i(\mathbf{D}_1 - \mathbf{D}_2) & \mathbf{D}_1 + \mathbf{D}_2 \end{bmatrix} \quad (\text{VI.15})$$

For any  $j \in \{1, \dots, n\}$ , define

$$\Sigma_j = \frac{1}{2}(\mathbf{D}_1 + \mathbf{D}_2)_{jj} = \frac{\mu_j - \mu_{n+j}}{2} > 0 \quad (\text{VI.16})$$

and

$$\Delta_j = \frac{1}{2}(\mathbf{D}_1 - \mathbf{D}_2)_{jj} = \frac{\mu_j + \mu_{n+j}}{2} \quad (\text{VI.17})$$

and let  $\Sigma = \text{diag}(\Sigma_1, \dots, \Sigma_n) \geq 0$  and  $\Delta = \text{diag}(\Delta_1, \dots, \Delta_n)$ . Injecting into Eqs. (VI.13) and (VI.15), we obtain

$$\bar{\mathbf{S}} = \mathbf{M} \begin{bmatrix} \Sigma & i\Delta \\ -i\Delta & \Sigma \end{bmatrix} \mathbf{M}^\dagger \quad (\text{VI.18})$$

which concludes the proof.  $\square$

### B. Proof of Theorem 4 of main text

At this stage, Theorem 12 has laid out the matrix form of Theorem 4, but we still need to incorporate the uncertainty principle on each  $\Sigma_j[\omega]$  and  $\Delta_j[\omega]$ . We first recall some handy mathematical results in the following two lemmas, whose proofs are straightforward.

**Lemma 2.** *A block-diagonal matrix is  $HP(S)D$  if and only if each of its diagonal block is  $HP(S)D$ . Similarly, for a matrix  $\mathbf{B}$  of the form  $\mathbf{B} = \begin{bmatrix} \mathbf{S} & i\mathbf{D} \\ -i\mathbf{D} & \mathbf{S} \end{bmatrix}$  with diagonal matrices  $\mathbf{S} = \text{diag}(S_1, \dots, S_n)$  and  $\mathbf{D} = \text{diag}(D_1, \dots, D_n)$ ,  $\mathbf{B}$  is  $HP(S)D$  if and only if for any  $j \in \{1, \dots, n\}$ , the  $2 \times 2$  matrix  $\begin{bmatrix} S_j & iD_j \\ -iD_j & S_j \end{bmatrix}$  is  $HP(S)D$ .*

**Lemma 3.** *Let  $\mathbf{A}(\Sigma, \Delta) = \begin{bmatrix} \Sigma & i\Delta \\ -i\Delta & \Sigma \end{bmatrix}$  with  $\Sigma, \Delta \in \mathbb{R}$ . Then:*

1. *The eigenvalues of  $\mathbf{A}(\Sigma, \Delta)$  are  $\Sigma \pm \Delta$ .*
2. *The eigenvalues of  $(\mathbf{A}(\Sigma, \Delta) + i\mathbf{J}/2)$  are  $\Sigma \pm (\Delta + \frac{1}{2})$ .*

The proof of Theorem 4 of the main text follows from Theorem 12 and these lemmas.

*Proof of Theorem 4.* Let  $\bar{\mathbf{S}}$  the SDM of some  $n$ -mode quantum system. According to Section V, it is HPD so Theorem 12 applies. We choose to apply it for all  $\omega \geq 0$ . There exists  $\mathbf{M}[\omega] \in \text{Sp}^\dagger(2n)$ , a real positive diagonal matrix  $\Sigma[\omega] = \text{diag}(\Sigma_1[\omega], \dots, \Sigma_n[\omega]) > 0$ , a real (not necessarily positive) diagonal matrix  $\Delta[\omega] = \text{diag}(\Delta_1[\omega], \dots, \Delta_n[\omega])$  such that

$$\bar{\mathbf{S}}[\omega] = \mathbf{M}[\omega] \begin{bmatrix} \Sigma[\omega] & i\Delta[\omega] \\ -i\Delta[\omega] & \Sigma[\omega] \end{bmatrix} \mathbf{M}[\omega]^\dagger \quad (\text{VI.19})$$

Since  $\bar{\mathbf{S}}[\omega]^* = \bar{\mathbf{S}}[-\omega]$ , we can construct the matrices  $\mathbf{M}[\omega]$ ,  $\Sigma[\omega]$  and  $\Delta[\omega]$  for the negative frequencies:  $\forall \omega < 0$ ,

$$\mathbf{M}[\omega] := \mathbf{M}[-\omega]^*, \quad \Sigma[\omega] := \Sigma[-\omega], \quad \Delta[\omega] := -\Delta[-\omega] \quad (\text{VI.20})$$

Finally, the case  $\omega = 0$ , where  $\bar{\mathbf{S}}[\omega]$  is real-valued, is a direct consequence of the Williamson theorem (Theorem 11), for which  $\mathbf{M}[0] \in \text{Sp}(2n, \mathbb{R})$  and  $\Delta[0] = \mathbf{0}$  still satisfies the properties of Eq. (VI.20). Doing so allows to extend the Williamson decomposition Eq. (VI.19) to any  $\omega \in \mathbb{R}$ . We now need to show that the uncertainty principle implies the constraints of Eq. (40) on the entries of  $\Sigma[\omega]$  and  $\Delta[\omega]$ . The uncertainty principle applied to the form of Eq. (VI.19) reads that for any frequency  $\omega$ , the matrix

$$\bar{\mathbf{S}}[\omega] + \frac{i\mathbf{J}}{2} = \mathbf{M}[\omega] \begin{bmatrix} \Sigma[\omega] & i(\Delta[\omega] + \frac{1_n}{2}) \\ -i(\Delta[\omega] + \frac{1_n}{2}) & \Sigma[\omega] \end{bmatrix} \mathbf{M}[\omega]^\dagger \quad (\text{VI.21})$$

is HPSD.

Since  $\mathbf{M}[\omega]$  is invertible, we can apply Proposition 1 to obtain that

$$\begin{bmatrix} \mathbf{\Sigma}[\omega] & i(\mathbf{\Delta}[\omega] + \frac{1}{2}) \\ -i(\mathbf{\Delta}[\omega] + \frac{1}{2}) & \mathbf{\Sigma}[\omega] \end{bmatrix} \quad \text{is HPD.} \quad (\text{VI.22})$$

Due to Lemmas 2 and 3, this requires that,  $\forall \omega \in \mathbb{R}, \forall j \in \{1, \dots, n\}$ ,  $\Sigma_j[\omega] - \Delta_j[\omega] - \frac{1}{2} \geq 0$ . Evaluating this at  $-\omega$  and using the parities of  $\Sigma_j[\omega]$  and  $\Delta_j[\omega]$  derived in Eq. (VI.20) yields  $\Sigma_j[\omega] + \Delta_j[\omega] - \frac{1}{2} \geq 0$ . Combining these two inequalities, we thus see that

$$\forall \omega \in \mathbb{R}, \quad \Sigma_j[\omega] \geq |\Delta_j[\omega]| + \frac{1}{2} \quad (\text{VI.23})$$

which concludes the proof.  $\square$

## VII. PROOF OF THE TIGHTER UNCERTAINTY BOUND FOR OPEN LTI SYSTEMS (THEOREM 5 OF MAIN TEXT)

We recall Theorem 5 of the main text and provide its proof:

**Theorem.** *Assuming that the noise modes (i.e. inaccessible inputs) are uncorrelated with each other and with the input modes, the output modes' spectral densities satisfy, for all  $i \in \{1, \dots, n\}$*

$$\sqrt{\bar{S}_{q_i q_i} \bar{S}_{p_i p_i}} \geq \left( \det \sum_{j,k} \mathbf{G}_{ij} \bar{\mathbf{S}}_{jk}^{in} \mathbf{G}_{ki}^\dagger \right)^{1/2} + \frac{1}{2} \sum_j \det |\mathbf{N}_{ij}|. \quad (\text{VII.1})$$

where the matrices on the right hand side are defined as: for  $\mathbf{A} \in \{\mathbf{G}, \bar{\mathbf{S}}^{in}, \mathbf{N}\}$ ,

$$\mathbf{A}_{jk} := \begin{bmatrix} A_{q_j q_k} & A_{q_j p_k} \\ A_{p_j q_k} & A_{p_j p_k} \end{bmatrix}. \quad (\text{VII.2})$$

*Proof.* Assuming that the accessible and inaccessible inputs are uncorrelated, the input-output relation in Eq. (52) implies (qualitatively comparable to the first term in Eq. (44) of main text)

$$\bar{\mathbf{S}}^{\text{out}}[\omega] = \mathbf{G}[\omega] \bar{\mathbf{S}}^{\text{in}}[\omega] \mathbf{G}[\omega]^\dagger + \mathbf{N}[\omega] \bar{\mathbf{S}}^{\text{N}}[\omega] \mathbf{N}[\omega]^\dagger. \quad (\text{VII.3})$$

One way to characterize the system's output fluctuations is to focus on the uncertainty between the quadratures of a single output quantum noise. This can be done by considering the  $2 \times 2$  block matrices that make up  $\bar{\mathbf{S}}^{\text{out}}$ :

$$\bar{\mathbf{S}}^{\text{out}} := \begin{bmatrix} \bar{\mathbf{S}}_{11}^{\text{out}} & \cdots & \bar{\mathbf{S}}_{1n}^{\text{out}} \\ \vdots & \ddots & \vdots \\ \bar{\mathbf{S}}_{n1}^{\text{out}} & \cdots & \bar{\mathbf{S}}_{nn}^{\text{out}} \end{bmatrix}, \quad (\text{VII.4})$$

where

$$\bar{\mathbf{S}}_{ii}^{\text{out}} := \begin{bmatrix} \bar{S}_{q_i q_i}^{\text{out}} & \bar{S}_{q_i p_i}^{\text{out}} \\ \bar{S}_{p_i q_i}^{\text{out}} & \bar{S}_{p_i p_i}^{\text{out}} \end{bmatrix}. \quad (\text{VII.5})$$

Note that in Eqs. (VII.4) and (VII.5), and in the rest of this section, we assume that the spectral density and transfer function matrices are written using the ordering  $\{\hat{q}_1, \hat{p}_1, \dots, \hat{q}_n, \hat{p}_n\}$  rather than  $\{\hat{q}_1, \dots, \hat{q}_n, \hat{p}_1, \dots, \hat{p}_n\}$  used in the rest of the paper. With this convention, the SDM of the  $i^{\text{th}}$  output mode is

$$\bar{\mathbf{S}}_{ii}^{\text{out}} = \sum_{j,k} \left[ \mathbf{G}_{ij} \bar{\mathbf{S}}_{jk}^{\text{in}} \mathbf{G}_{ki}^\dagger + \mathbf{N}_{ij} \bar{\mathbf{S}}_{jk}^{\text{N}} \mathbf{N}_{ki}^\dagger \right]. \quad (\text{VII.6})$$

We now assume that the noise modes are uncorrelated with each other and with the input modes,  $\bar{\mathbf{S}}_{jk}^{\text{N}} = 0$  unless  $j = k$ . This assumption allows us to bound the output spectral densities of the  $i^{\text{th}}$  output mode as follows. First note

that  $\sqrt{\bar{S}_{q_i q_i}^{\text{out}} \bar{S}_{p_i p_i}^{\text{out}}} \geq (\det \bar{S}_{ii}^{\text{out}})^{1/2}$ ; then the strategy is to insert the above expression for  $\bar{S}_{ii}^{\text{out}}$  and use the Minkowski inequality to lower-bound the determinant of the sum. Note that the Minkowski inequality (Theorem 7.8.21 of Ref. [2]) states that for a pair of  $n \times n$  matrices,  $(\det(A+B))^{1/n} \geq (\det A)^{1/n} + (\det B)^{1/n}$ . This implies that for a collection of  $N$   $n \times n$  matrices  $M_i$ , by repeated application of the basic Minkowski inequality:

$$\begin{aligned}
\left( \det \left( \sum_{i=1}^N M_i \right) \right)^{1/n} &= \left( \det \left( M_1 + \sum_{i=2}^N M_i \right) \right)^{1/n} \\
&\geq (\det(M_1))^{1/n} + \left( \det \left( \sum_{i=2}^N M_i \right) \right)^{1/n} \\
&\geq \dots \\
&\geq (\det(M_1))^{1/n} + (\det(M_2))^{1/n} \\
&\quad + \dots + (\det(M_N))^{1/n} \\
&\geq \sum_{i=1}^N (\det(M_i))^{1/n}.
\end{aligned} \tag{VII.7}$$

Applying this to Eq. (VII.6) gives

$$\sqrt{\bar{S}_{q_i q_i}^{\text{out}} \bar{S}_{p_i p_i}^{\text{out}}} \geq \left( \det \sum_{j,k} \mathbf{G}_{ij} \bar{\mathbf{S}}_{jk}^{\text{in}} \mathbf{G}_{ki}^\dagger \right)^{1/2} + \sum_j \left( \det \mathbf{N}_{ij} \bar{\mathbf{S}}_{jj}^{\text{N}} \mathbf{N}_{ji}^\dagger \right)^{1/2}. \tag{VII.8}$$

Finally employing the multiplicative property of the determinant, and the uncertainty principle [Eq. (39)],  $\det(\bar{\mathbf{S}}_{jj}^{\text{N}}) \geq 1/4$ , gives

$$\sqrt{\bar{S}_{q_i q_i}^{\text{out}} \bar{S}_{p_i p_i}^{\text{out}}} \geq \left( \det \sum_{j,k} \mathbf{G}_{ij} \bar{\mathbf{S}}_{jk}^{\text{in}} \mathbf{G}_{ki}^\dagger \right)^{1/2} + \frac{1}{2} \sum_j |\det \mathbf{N}_{ij}|. \tag{VII.9}$$

□

## VIII. THE SYNODYNE DETECTION LOCAL OSCILLATOR AS AN EXAMPLE OF QUADRATURE AMPLITUDE MODULATION (SECTION V A OF MAIN TEXT)

In this appendix, we revisit the local oscillator choice for synodyne detection (Eq. (61) of main text) through the prism of signal modulation.

We hope that such clarification paves the way for a better understanding of the effect of local oscillator modulation on the measured quantum quadratures and bridges the gap between multimode quantum optics and classical signal processing [12–14].

### A. Quadrature amplitude modulation

Consider a sinusoidal (real-valued) carrier field  $E_c(t) = E_0 \cos(\omega_\ell t + \phi_0)$ , which can be rewritten in the quadrature form  $E_c(t) = E_{c0} \cos(\omega_\ell t) + E_{s0} \sin(\omega_\ell t)$ . Quadrature amplitude modulation consists in changing  $E_{c0}$  and  $E_{s0}$  over time, on a typical timescale usually much slower than  $1/\omega_\ell$ . Let us consider the case of a carrier-less sinusoidal modulation where  $E_{c0} \mapsto A_1 \cos(\omega_1 t + \phi_1)$  and  $E_{s0} \mapsto A_2 \cos(\omega_2 t + \phi_2)$  with  $0 < \omega_1, \omega_2 \ll \omega_\ell$ . The modulation on  $E_{c0}$  is also known as amplitude modulation, while the one on  $E_{s0}$  is called phase modulation.

In the special case where  $\omega_1 = \omega_2$ , the field after QAM reads in the frequency domain

$$E_{\text{QAM}}[\omega > 0] = \pi(A_1 e^{-i\phi_1} + iA_2 e^{-i\phi_2})\delta[\omega - (\omega_\ell + \omega_1)] + \pi(A_1 e^{i\phi_1} + iA_2 e^{i\phi_2})\delta[\omega - (\omega_\ell - \omega_1)] \tag{VIII.1}$$

and since  $E(t)$  is real, we recover the negative frequency components with  $E_{\text{QAM}}[-\omega] = E_{\text{QAM}}[\omega]^*$ .

### B. Connection with the synodyne local oscillator

Recall that the synodyne local oscillator has the complex form  $\alpha[\omega] = \sqrt{2\pi}\{(\alpha_{q0} + i\alpha_{p0})\delta[\omega - \omega_0] + (\alpha_{q0}^* + i\alpha_{p0}^*)\delta[\omega + \omega_0]\}$ . The time-domain electric field for the synodyne local oscillator thus has the form  $E^{\text{SD}}(t) = \alpha(t)e^{-i\omega_\ell t} + \alpha^*(t)e^{i\omega_\ell t}$ , where  $\omega_\ell$  is the frequency of the carrier and  $\alpha(t) = \frac{\alpha_{q0} + i\alpha_{p0}}{\sqrt{2}}e^{-i\omega_0 t} + \frac{\alpha_{q0}^* + i\alpha_{p0}^*}{\sqrt{2}}e^{i\omega_0 t}$ . Its Fourier transform is

$$E^{\text{SD}}[\omega > 0] = \sqrt{2\pi}\{(\alpha_{q0}^{\text{SD}} + i\alpha_{p0}^{\text{SD}})\delta[\omega - (\omega_\ell + \omega_0)] + (\alpha_{q0}^{\text{SD}*} + i\alpha_{p0}^{\text{SD}*})\delta[\omega - (\omega_\ell - \omega_0)]\} \quad (\text{VIII.2})$$

Comparing Eq. (VIII.1) with Eq. (VIII.2), we identify the synodyne local oscillator as a carrier-less QAM, that is,  $\omega_0 \rightarrow \omega_1$ ,  $\sqrt{2}\alpha_{q0}^{\text{SD}} \rightarrow A_1 e^{-i\phi_1}$  and  $\sqrt{2}\alpha_{p0}^{\text{SD}} \rightarrow A_2 e^{-i\phi_2}$ . In other words, the synodyne local oscillator is a superposition of amplitude and phase modulations at the same frequency  $\omega_0$  with suppressed carrier.

### IX. AN EXAMPLE OF A FREQUENCY-DEPENDENT TWO-MODE BEAMSPLITTER (SECTION VIA OF MAIN TEXT)

In this appendix we provide an optical example of a frequency-dependent beamsplitter, as studied in Section VIA of the main text, in the form of a lossless Fabry-Perot cavity made of two mirrors with different reflectivities. We denote by  $(r_1, t_1)$  and  $(r_2, t_2)$  the reflection and transmission coefficients of the two mirrors, and choose the convention that they are all positive, but the reflections on the internal sides of the cavity have a  $\pi$  phase shift. Since the total power is conserved, one has  $r_1^2 + t_1^2 = r_2^2 + t_2^2 = 1$  and since the mirrors are passive, it suffices work with the annihilation operators at a given frequency  $\omega$ . For the two input modes  $(\hat{a}_{\text{in}1}[\omega], \hat{a}_{\text{in}2}[\omega])$  and outputs  $(\hat{a}_{\text{out}1}[\omega], \hat{a}_{\text{out}2}[\omega])$ , the transfer matrix through the cavity is

$$\begin{bmatrix} \hat{a}_{\text{out}1}[\omega] \\ \hat{a}_{\text{out}2}[\omega] \end{bmatrix} = \begin{bmatrix} F_{11}[\omega] & F_{12}[\omega] \\ F_{21}[\omega] & F_{22}[\omega] \end{bmatrix} \begin{bmatrix} \hat{a}_{\text{in}1}[\omega] \\ \hat{a}_{\text{in}2}[\omega] \end{bmatrix} \quad (\text{IX.1})$$

where

$$F_{11}[\omega] = \frac{r_1 - r_2 e^{2i\phi[\omega]}}{1 - r_1 r_2 e^{2i\phi[\omega]}}, \quad F_{12}[\omega] = \frac{t_1 t_2 e^{i\phi[\omega]}}{1 - r_1 r_2 e^{2i\phi[\omega]}} \quad (\text{IX.2})$$

with  $\phi[\omega] = (\omega_0 + \omega)L/c$ , where  $L$  is the half round trip length of the cavity. The matrix elements  $F_{21}$  and  $F_{22}$  are obtained from  $F_{12}$  and  $F_{11}$  respectively by exchanging the indices 1 and 2 for the mirror coefficients. One notices that  $F_{12}[\omega] = F_{21}[\omega]$  and that  $|F_{22}[\omega]| = |F_{11}[\omega]|$ . As a sanity check, one can verify that the matrix  $\mathbf{F}[\omega] = (F_{ij}[\omega])_{i,j \in \{1,2\}}$  thus defined is unitary for all frequencies, which means that it is both a passive transformation and that the corresponding transformation on the quadratures is symplectic. To simplify, we assume that  $\omega_0 L/c = 0 \bmod (2\pi)$ , so that  $\mathbf{F}[-\omega]^\dagger = \mathbf{F}[\omega]$ . Then, the corresponding symplectic matrix on the quadratures has the block diagonal form

$$\hat{\mathbf{x}}_{\text{out}}[\omega] = \begin{bmatrix} \mathbf{F}[\omega] & \mathbf{0}_{2 \times 2} \\ \mathbf{0}_{2 \times 2} & \mathbf{F}[\omega] \end{bmatrix} \hat{\mathbf{x}}_{\text{in}}[\omega] \quad (\text{IX.3})$$

Through direct computation, one finds

$$\mathbf{F}[\omega] = \begin{bmatrix} e^{i\phi_{11}} & 0 \\ 0 & e^{i\phi_{22}} \end{bmatrix} \begin{bmatrix} \cos(\alpha) & -\sin(\alpha)e^{i\beta} \\ \sin(\alpha)e^{-i\beta} & \cos(\alpha) \end{bmatrix} = \begin{bmatrix} \cos(\alpha) & -\sin(\alpha)e^{i\beta'} \\ \sin(\alpha)e^{-i\beta'} & \cos(\alpha) \end{bmatrix} \begin{bmatrix} e^{i\phi_{11}} & 0 \\ 0 & e^{i\phi_{22}} \end{bmatrix} \quad (\text{IX.4})$$

where all the matrix coefficients depend on  $\omega$  (omitted for clarity) and are defined as

$$\phi_{jk}[\omega] = \arg(F_{jk}[\omega]) \quad \forall j, k \in \{1, 2\} \quad (\text{IX.5})$$

$$\cos(\alpha[\omega]) = |F_{11}[\omega]| \quad (\text{IX.6})$$

$$\sin(\alpha[\omega]) = |F_{21}[\omega]| \quad (\text{IX.7})$$

$$\beta[\omega] = \phi_{22}[\omega] - \phi_{12}[\omega] = \phi_{12}[\omega] - \phi_{11}[\omega] \pm \pi \quad (\text{IX.8})$$

$$\beta'[\omega] = -\beta[\omega] \quad (\text{IX.9})$$

When  $r_1 \neq r_2$ , the phase  $\beta$  explicitly depends on  $\omega$  as  $\beta[\omega] = \phi[\omega] - \arg(r_2 - r_1 e^{2i\phi[\omega]})$ . Therefore, comparing Eqs. (IX.3) and (IX.4) with the general form of a frequency-dependent beam-splitter

$$\begin{bmatrix} \mathbf{U} & \mathbf{0} \\ \mathbf{0} & \mathbf{U} \end{bmatrix} = \begin{bmatrix} \cos \alpha & -e^{i\beta} \sin \alpha & 0 & 0 \\ e^{-i\beta} \sin \alpha & \cos \alpha & 0 & 0 \\ 0 & 0 & \cos \alpha & -e^{i\beta} \sin \alpha \\ 0 & 0 & e^{-i\beta} \sin \alpha & \cos \alpha \end{bmatrix}, \quad (\text{IX.10})$$

we have shown that any non-critically coupled Fabry-Perot interferometer constitutes a non-trivial example of a frequency-dependent beamsplitter (i.e. it has complex-valued elements  $e^{\pm i\beta}$  which cannot be canceled by a phase reference choice, unlike  $\phi_{11}$  and  $\phi_{22}$ ).

It is worth noting that one can approximate a two mode frequency-dependent beamsplitter of arbitrary coefficients  $\alpha[\omega]$  and  $\beta[\omega]$  by nesting Fabry-Perot cavities, or by putting them in series.

## X. DETAILS OF COMPLEX SQUEEZING IN LOSSY PASSIVE SYSTEMS (SECTION VIB OF MAIN TEXT)

We provide details to the derivation of complex squeezing in lossy systems, Section VIB of main text.

### A. Derivation of the output SDM of equation 64 in main text

We recall that we consider a passive system acting on a single input mode  $\hat{\mathbf{a}}_{\text{in}}[\omega] = [\hat{a}_{\text{in}}[\omega], \hat{a}_{\text{in}}[-\omega]^\dagger]^T$ , whose transfer function between observable inputs and outputs is  $F[\omega]$ , In other words, the classical input-output relation is

$$a_{\text{out}}[\omega] = F[\omega] a_{\text{in}}[\omega] \quad (\text{X.1})$$

By direct computation (appendix C of [15]), the corresponding transfer function matrix  $\mathbf{G}[\omega]$  in the quadrature basis has the form  $\mathbf{x}_{\text{out}}[\omega] = \mathbf{G}[\omega] \mathbf{x}_{\text{in}}[\omega]$ , where

$$\mathbf{G}[\omega] = e^{i\theta_C} \left[ C\mathbf{R}(\theta_D) + iD\mathbf{R}\left(\theta_D - \frac{\pi}{2}\right) \right] \quad (\text{X.2})$$

with

$$C[\omega] = \frac{|F[\omega]| + |F[-\omega]|}{2}, \quad D[\omega] = \frac{|F[\omega]| - |F[-\omega]|}{2}, \quad (\text{X.3})$$

$$\theta_C[\omega] = \frac{\arg(F[\omega]) - \arg(F[-\omega])}{2}, \quad \theta_D[\omega] = \frac{\arg(F[\omega]) + \arg(F[-\omega])}{2} \quad (\text{X.4})$$

and the explicit dependency in  $\omega$  has been omitted in Eq. (X.2) for simplicity.

Since we are considering a lossy passive system, we have  $|F[\omega]| < 1$  and to preserve the commutation relations, it suffices to promote Eq. (X.1) to a valid operator relation by adding a single additional mode:  $\hat{a}_{\text{out}}[\omega] = F[\omega] \hat{a}_{\text{in}}[\omega] + L[\omega] \hat{a}_{\text{vac}}[\omega]$  where  $\hat{a}_{\text{vac}}$  is an external noise mode (taken here to be vacuum) and  $L[\omega]$  is its transfer function to the signal output. Define the functions  $C_L[\omega], D_L[\omega], \theta_{CL}[\omega]$  and  $\theta_{DL}[\omega]$  similarly to Eq. (X.3), and  $\mathbf{H}_L[\omega]$  similarly to Eq. (X.2), by replacing  $F[\omega]$  with  $L[\omega]$ . One then obtains the input-output relation on the quadratures  $\hat{\mathbf{x}}_{\text{out}}[\omega] = \mathbf{G}[\omega] \hat{\mathbf{x}}_{\text{in}}[\omega] + \mathbf{G}_L[\omega] \hat{\mathbf{x}}_{\text{vac}}[\omega]$ . Imposing that the output quadratures preserve the CCR is equivalent to having  $|F[\omega]|^2 + |L[\omega]|^2 = 1$  which, in turn, can be recast in the quadrature picture as [16]  $\mathbf{G}[\omega] \mathbf{G}[\omega]^\dagger + \mathbf{G}_L[\omega] \mathbf{G}_L[\omega]^\dagger = \mathbf{1}$ . This simplifies the expression of the output SDM which is  $\bar{\mathbf{S}}_{\text{out}}[\omega] = \mathbf{G}[\omega] \bar{\mathbf{S}}_{\text{in}}[\omega] \mathbf{G}[\omega]^\dagger + \mathbf{G}_L[\omega] \bar{\mathbf{S}}_{\text{vac}}[\omega] \mathbf{G}_L[\omega]^\dagger$ . Thus

$$\bar{\mathbf{S}}_{\text{out}}[\omega] = \mathbf{G}[\omega] \bar{\mathbf{S}}_{\text{in}}[\omega] \mathbf{G}[\omega]^\dagger + \frac{\mathbf{1} - \mathbf{G}[\omega] \mathbf{G}[\omega]^\dagger}{2} = \mathbf{G}[\omega] \left( \bar{\mathbf{S}}_{\text{in}}[\omega] - \frac{\mathbf{1}}{2} \right) \mathbf{G}[\omega]^\dagger + \frac{\mathbf{1}}{2} \quad (\text{X.5})$$

and because  $\mathbf{G}[\omega]$  is complex-valued as soon as  $D \neq 0$  (Eq. (X.2)), in other words when the system presents a sideband asymmetry due to loss, we see that  $\bar{\mathbf{S}}_{\text{out}}[\omega]$  also becomes complex-valued in general. Substituting  $\mathbf{G}[\omega]$  in this equation and simplifying the elements yields Eq. (64) of the main text.

### B. Full expressions of the eigenvalues $\Lambda_-^{\mathbb{R}, \mathbb{C}}$

We can analytically diagonalize the output SDM of Eq. (64) of the main text as well as its elementwise real part to obtain the following expressions for their smaller eigenvalue:

$$\Lambda_-^{\mathbb{C}} = \min_{\alpha \in \mathbb{C}^2} \frac{\alpha^\dagger \bar{\mathbf{S}}_{\text{out}}[\omega] \alpha}{\alpha^\dagger \alpha} = \frac{1}{2} + \frac{1}{2} \left[ (F_+^2 + F_-^2) \sinh^2(r) - \sinh(2r) F_+ F_- \sqrt{1 + \frac{\tanh^2(r) (F_-^2 - F_+^2)^2}{4F_-^2 F_+^2}} \right] \quad (\text{X.6})$$

$$\Lambda_-^{\mathbb{R}} = \min_{\alpha \in \mathbb{C}^2} \frac{\alpha^\dagger \text{Re}(\bar{\mathbf{S}}_{\text{out}}[\omega]) \alpha}{\alpha^\dagger \alpha} = \frac{1}{2} + \frac{1}{2} [(F_+^2 + F_-^2) \sinh^2(r) - \sinh(2r) F_+ F_-] \quad (\text{X.7})$$

### C. Validity of the approximation of main text Eq. 66

We seek an approximate form for  $\Lambda_-^C$  which is comparable to the usual frequency-independent interpretation of a lossy system modeled as a beamsplitter. Recall that the output quantum noise  $N_{FI}$  relative to vacuum ( $1/2$ ), measured on the squeezed quadrature, for a frequency-dependent lossy system, is written as  $N_{FI} = (1 - \eta) + \eta e^{-2r}$  where  $\eta$  is the transmission efficiency of the squeezed state propagation.

In the limit of large squeezing  $r \rightarrow \infty$ , one can expand Eq. (X.6) at the lowest order in  $e^{-2r}$  and find an equivalent efficiency  $\eta^C \in [0, 1]$  given by the harmonic mean of the sideband efficiencies:

$$\eta^C[\omega] = \frac{2F_-^2 F_+^2}{F_-^2 + F_+^2} = \frac{2}{\frac{1}{F_-^2} + \frac{1}{F_+^2}} \quad (\text{X.8})$$

such that

$$\Lambda_-^C \underset{r \rightarrow \infty}{=} \frac{1}{2} [(1 - \eta^C) + \eta^C e^{-2r}] =: \Lambda_\infty^C \quad (\text{X.9})$$

Surprisingly enough, while this equation is only valid at large squeezing, we numerically observe that it stays close to the exact expression of Eq. (X.6) for all squeezing values  $r > 0$ , as shown in figure Fig. 1. We numerically see that the relative discrepancy between  $\Lambda_\infty^C$  and  $\Lambda_-^C$  is bounded over all values of  $F_\pm \in [0, 1]^2$  by  $\simeq 4.3\%$ , or 0.183 dB.

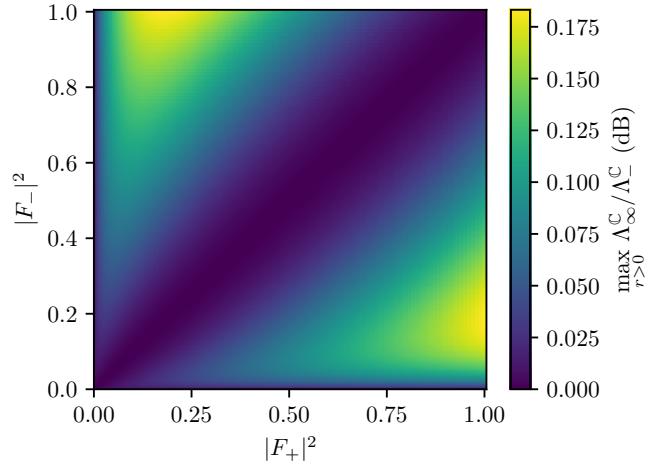

FIG. 1: Numerical comparison of the approximated optimal synodyne squeezing level ( $\Lambda_\infty^C$ , Eq. (X.9)) to the exact expression ( $\Lambda_-^C$ , Eq. (X.6)). This figure is made as follows: for each value of the sideband efficiency  $(F_+^2, F_-^2) \in [0, 1]^2$ , we maximize the ratio  $\Lambda_\infty^C / \Lambda_-^C$  over  $r > 0$  (in practice, it is sufficient to compute it  $r \in [0, 3]$  and take the maximum, as  $\Lambda_\infty^C$  is defined to be the limit of  $\Lambda_-^C$  for large  $r$ ). The result is converted in dB units using the formula  $(\Lambda_\infty^C / \Lambda_-^C)_{\text{dB}} = 10 \log_{10}(\Lambda_\infty^C / \Lambda_-^C)$ .

This approximation, now valid for all values of  $r$ , allows us to conclude on the physical meaning of a symplectodyne-type measurement, as compared to a homodyne detection. When frequency-dependent losses are present in the system, i.e. the transmission efficiencies of the sidebands are asymmetric  $F_+^2 \neq F_-^2$ , the output squeezed state experiences a rotation of its squeezed quadrature in the complex plane, such that no rotation of the homodyne quadrature allows to fully recover the quantum correlations. Thus, only a measurement scheme which can separate the positive and negative sideband frequencies is able to recover it: under the optimal complex quadrature, we can map the two sideband efficiencies  $F_\pm^2$  into a single, beam-splitter-like efficiency  $\eta^C[\omega]$  (Eq. (X.8)) which determines the highest amount of quantum squeezing which can be measured at any frequency.

### D. Choosing the parameters for a detuned filter cavity

The reflectivity of a Fabry-Prot cavity with input and output mirrors reflectivities defined as  $r_1$  and  $r_2$  is

$$|F[\omega]|^2 = \frac{(r_1 - r_2)^2 + 4r_1r_2 \sin^2(\phi[\omega])}{(1 - r_1r_2)^2 + 4r_1r_2 \sin^2(\phi[\omega])} = \frac{4R \sin^2(\phi[\omega])}{(1 - R)^2 + 4R \sin^2(\phi[\omega])} \quad (\text{X.10})$$

We see that in the high-finesse, critically coupled limit  $r_1^2 = r_2^2 = R \rightarrow 1$ , one has  $|F[\omega]|^2 \simeq 4R \sin^2(\phi[\omega]) / (4R \sin^2(\phi[\omega])) = 1$  unless  $\sin^2(\phi[\omega])$  is of the same order of magnitude than  $(1 - R)^2$ . Fixing  $\phi_0 = \pi/4$  and  $F_- \in [0, 1)$ , a direct computation shows that at

$$\frac{\omega L}{c} = \frac{\pi}{4} - \arcsin \left( \frac{1 - R}{2\sqrt{R}} \frac{F_-}{\sqrt{1 - F_-^2}} \right) \quad (\text{X.11})$$

we have  $|F[-\omega_0]| = F_-$  and

$$|F[+\omega_0]| = 1 - \frac{(1 - R)^2}{8} + O((1 - R)^3) \xrightarrow{R \rightarrow 1} 1 \quad (\text{X.12})$$

which means that we can tune the value of  $F_-$  while keeping  $F_+$  arbitrarily close to 1. The cavity response of the parameters chosen in the main text ( $F_+^2 = 0.99$  and  $F_-^2 = 0.3$  with  $\phi_0 = 45$  deg,  $R = 0.8$  and  $\omega L_0/c = 40.8$  deg) is shown in figure Fig. 2 (a) while the optical setup is shown in figure Fig. 2 (b).

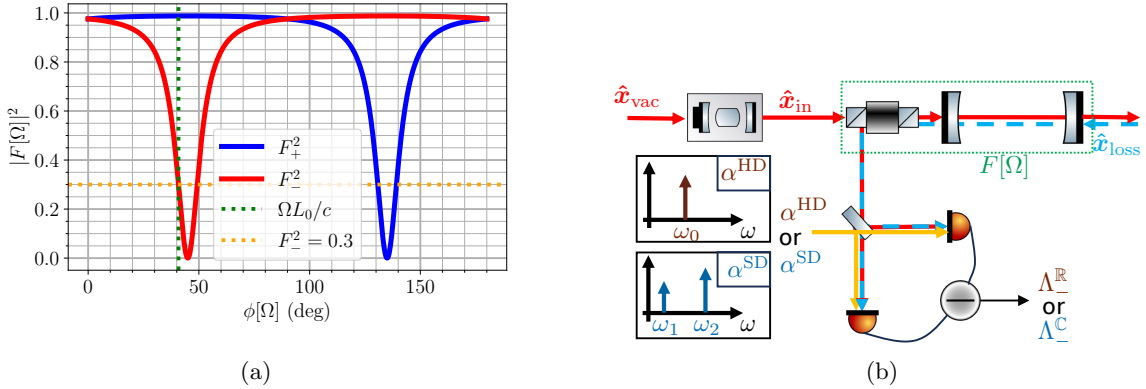

FIG. 2: (a) frequency response of a critically coupled lossy filter cavity, with  $R = 0.8$ . (b) Optical layout for generating complex squeezing and revealing its quantum nature by passing a broadband squeezed state through a critically coupled Fabry-Prot cavity and performing synodyne detection at its output. HD: homodyne detection; SD: synodyne detection.

## XI. DETAILS OF APPENDIX A OF MAIN TEXT

We detail some computations omitted in Appendix A of the main text.

**Theorem** (Change of basis for SDM). *The relation between  $\bar{S}^a[\omega]$  and  $\bar{S}[\omega]$  is*

$$\bar{S}[\omega] = \mathbf{P}^* \bar{S}^a[\omega] \mathbf{P}^T = \mathbf{P} \bar{S}^a[-\omega]^* \mathbf{P}^\dagger \quad (\text{XI.1})$$

*Proof.* For any  $j, k \in \{1, \dots, 2N\}$ ,

$$\bar{S}_{jk}[\omega] = \frac{1}{4\pi\delta[0]} \langle \hat{x}_j[\omega], \hat{x}_k[\omega]^\dagger \rangle = \frac{1}{4\pi\delta[0]} \langle \{P_{j\mu} \hat{a}_\mu[\omega], P_{k\nu}^* \hat{a}_\nu[\omega]^\dagger\} \rangle = \mathbf{P}_{j\mu} \frac{1}{4\pi\delta[0]} \langle \{\hat{a}_\mu[\omega], \hat{a}_\nu[\omega]^\dagger\} \rangle (\mathbf{P}^\dagger)_{\nu k} \quad (\text{XI.2})$$

But

$$\langle \{\hat{\mathbf{a}}_\mu[\omega], \hat{\mathbf{a}}_\nu[\omega]^\dagger\} \rangle = (\langle \hat{\mathbf{a}}_\mu[\omega] \hat{\mathbf{a}}_\nu[\omega]^\dagger + \hat{\mathbf{a}}_\nu[\omega]^\dagger \hat{\mathbf{a}}_\mu[\omega] \rangle^*)^* = \langle \{\hat{\mathbf{a}}_\mu[\omega]^\dagger, \hat{\mathbf{a}}_\nu[\omega]\} \rangle^* \quad (\text{XI.3})$$

So

$$\bar{S}_{jk}[\omega] = \mathbf{P}_{j\mu} \left( \frac{1}{4\pi\delta[0]} \langle \{\hat{\mathbf{a}}_\mu[\omega]^\dagger, \hat{\mathbf{a}}_\nu[\omega]\} \rangle \right)^* (\mathbf{P}^\dagger)_{\nu k} = \mathbf{P}_{j\mu} \bar{S}_{\mu\nu}^\alpha[-\omega]^* (\mathbf{P}^\dagger)_{\nu k} = \left( \mathbf{P} \bar{\mathbf{S}}^\alpha[-\omega]^* \mathbf{P}^\dagger \right)_{jk} \quad (\text{XI.4})$$

□

- 
- [1] J. A. Tropp, [ACM 204: Matrix Analysis, Caltech CMS Lecture Notes](#) (2022).
  - [2] R. A. Horn and C. R. Johnson, *Matrix Analysis*, 2nd ed. (Cambridge University Press, 2012).
  - [3] E. V. Haynsworth, Determination of the inertia of a partitioned hermitian matrix, [Linear Algebra and its Applications](#) **1**, 73 (1968).
  - [4] F. Caruso, J. Eisert, V. Giovannetti, and A. S. Holevo, Multi-mode bosonic gaussian channels, [New Journal of Physics](#) **10**, 083030 (2008).
  - [5] A. C. Silva, *Lectures on Symplectic Geometry*, edited by J.-M. Morel, F. Takens, and B. Teissier (Springer, 2008).
  - [6] B. Hoogenboom, *Intertwining functions on compact Lie groups* (Centrum voor Wiskunde en Informatica, 1984).
  - [7] A. Edelman and S. Jeong, Fifty three matrix factorizations: A systematic approach (2022), [arXiv:2104.08669 \[math.NA\]](#).
  - [8] H. Xu, An svd-like matrix decomposition and its applications, [Linear Algebra and its Applications](#) **368**, 1 (2003).
  - [9] É. Gouzien, *Optique quantique multimode pour le traitement de l'information quantique*, *Ph.D. thesis*, Université Côte d'Azur (2019).
  - [10] A. Knap, *Lie Groups: Beyond an Introduction*, 2nd ed. (Birkhauser, 2002).
  - [11] J. Williamson, On the algebraic problem concerning the normal forms of linear dynamical systems, [American Journal of Mathematics](#) **58**, 141 (1936).
  - [12] A. M. Marino, C. R. Stroud, Jr., V. Wong, R. S. Bennink, and R. W. Boyd, Bichromatic local oscillator for detection of two-mode squeezed states of light, [Journal of the Optical Society of America B](#) **24**, 335 (2007).
  - [13] W. Li, X. Yu, Z. Meng, Y. Jin, and J. Zhang, Experimental study of balanced optical homodyne and heterodyne detection by controlling sideband modulation, *Science China Physics* **58**, [10.1007/s11433-015-5718-z](#) (2015).
  - [14] W. Li, X. Yu, and J. Zhang, Measurement of the squeezed vacuum state by a bichromatic local oscillator, [Opt. Lett.](#) **40**, 5299 (2015).
  - [15] L. McCuller, S. E. Dwyer, A. C. Green, H. Yu, K. Kuns, *et al.*, LIGO's quantum response to squeezed states, [Phys. Rev. D](#) **104**, 062006 (2021).
  - [16] This is actually equivalent to Eq. (10) but much simpler to manipulate because  $\mathbf{J}$  does not appear. This is because we exploit the fact that all the matrices are diagonalized by  $\mathbf{P}$ , i.e. in the  $\mathbf{a}$  basis.
